# Supplementary material for: Feature-aware ultra-low dimensional reduction of real networks
Source: arXiv:2401.09368 source file (2024-06-10)
Supplement: Supplementary file 1 [file SI_compressed.pdf]

# Supplementary Information for "Feature-aware ultra-low dimensional reduction of real networks"

Robert Jankowski,[1,2] Pegah Hozhabrierdi,[3] Marián Boguñá,[1,2] and M. Ángeles Serrano[1,2,4,*]

[1] *Departament de Física de la Matèria Condensada, Universitat de Barcelona, Martí i Franquès 1, E-08028 Barcelona, Spain*

[2] *Universitat de Barcelona Institute of Complex Systems (UBICS), Universitat de Barcelona, Barcelona, Spain*

[3] *Department of Electrical Engineering and Computer Science, Syracuse University, 223 Link Hall, Syracuse, NY 13244*

[4] *ICREA, Passeig Lluís Companys 23, E-08010 Barcelona, Spain*

[*] marian.serrano@ub.edu

# I. SUPPLEMENTARY FIGURES

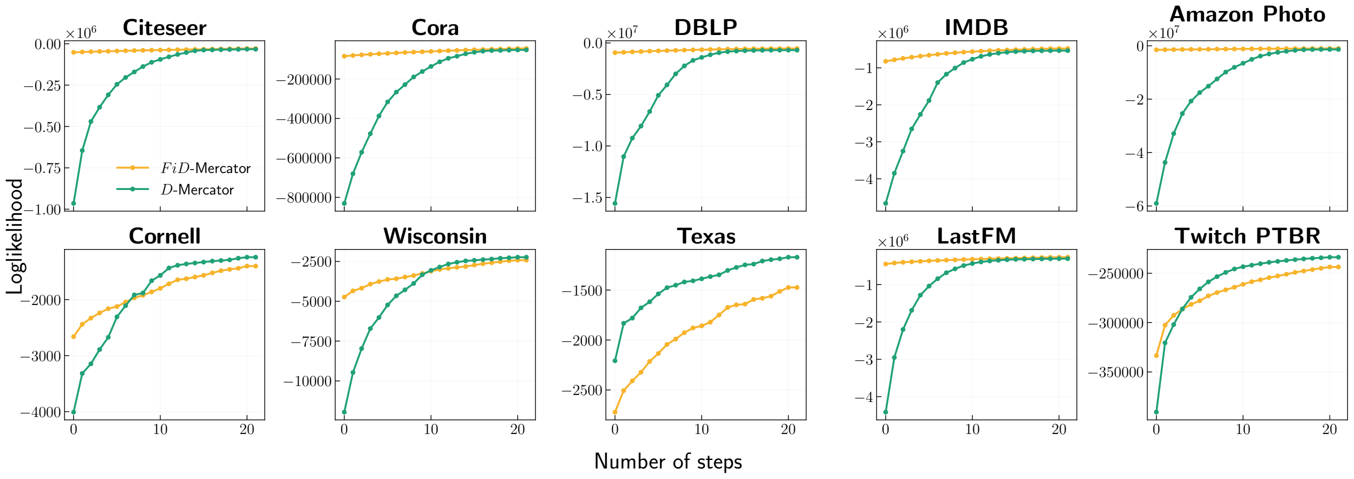


Supplementary Fig. 1: The evolution of the global loglikelihood during the maximum likelihood (ML) part.

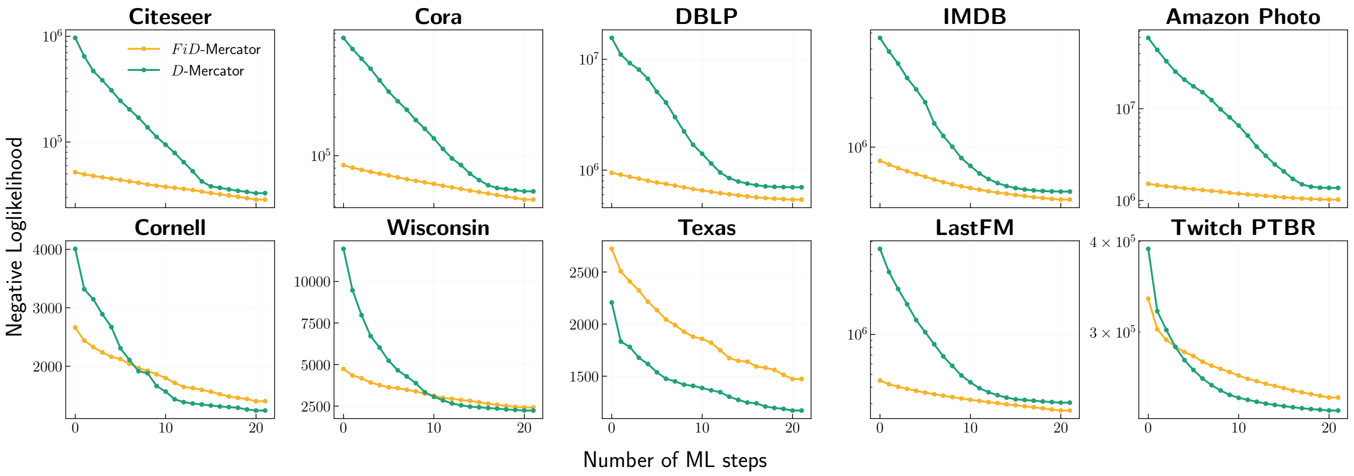


Supplementary Fig. 2: As in Supplementary Fig. 1, however the negative global loglikelihood is plotted in the log scale.

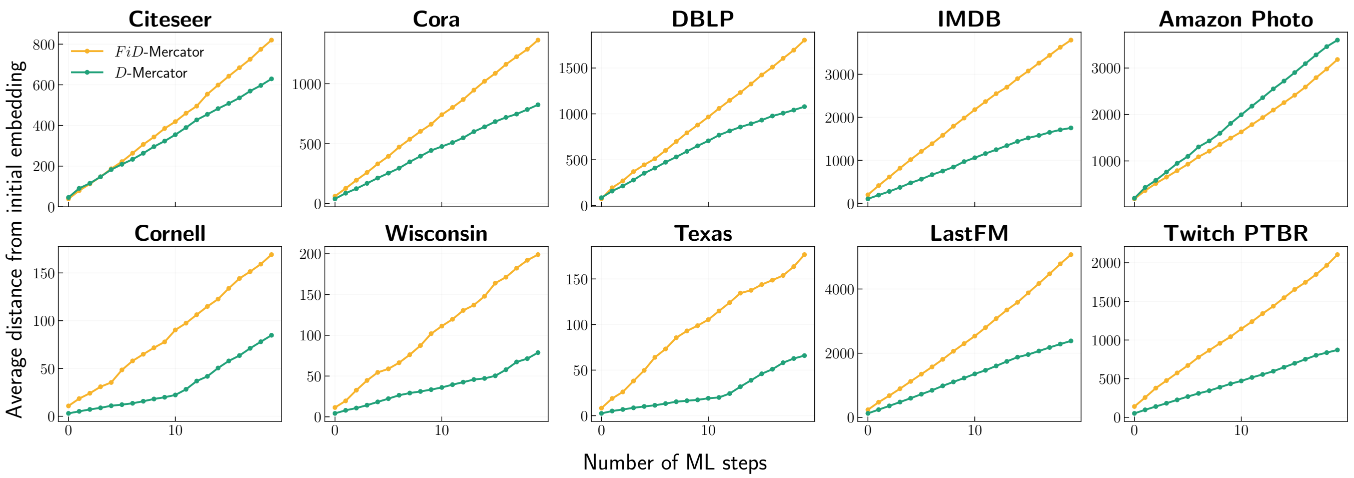


Supplementary Fig. 3: The average angular distance between each node of the initial embedding (for $D$-Mercator: Laplacian Eigenmaps; for $FiD$-Mercator: UMAP) and the embedding after each ML step.

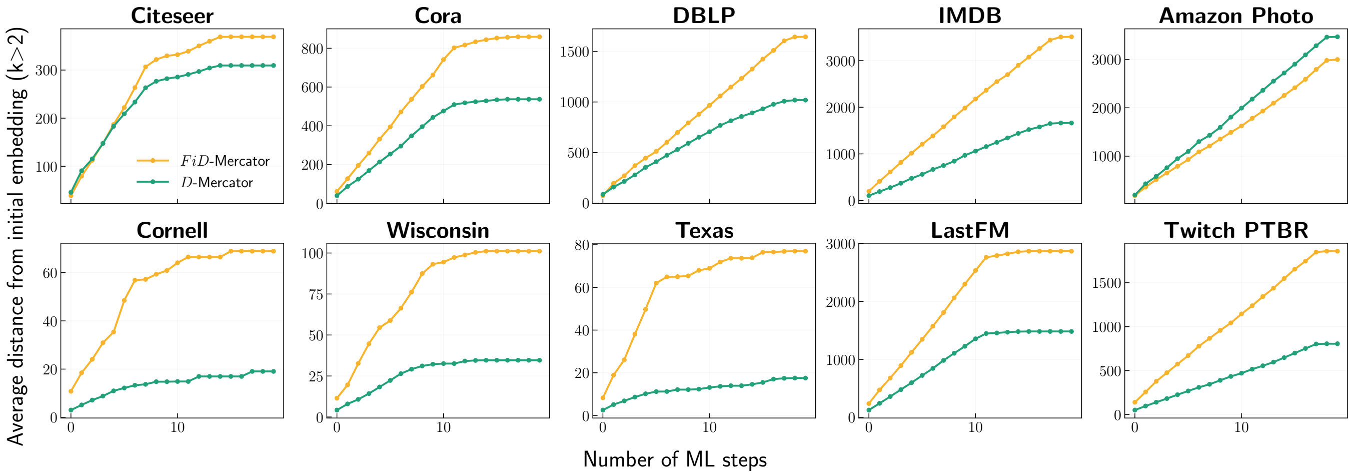


Supplementary Fig. 4: As in Supplementary Fig. 3, however the distance is computed only for nodes with $k > 2$.

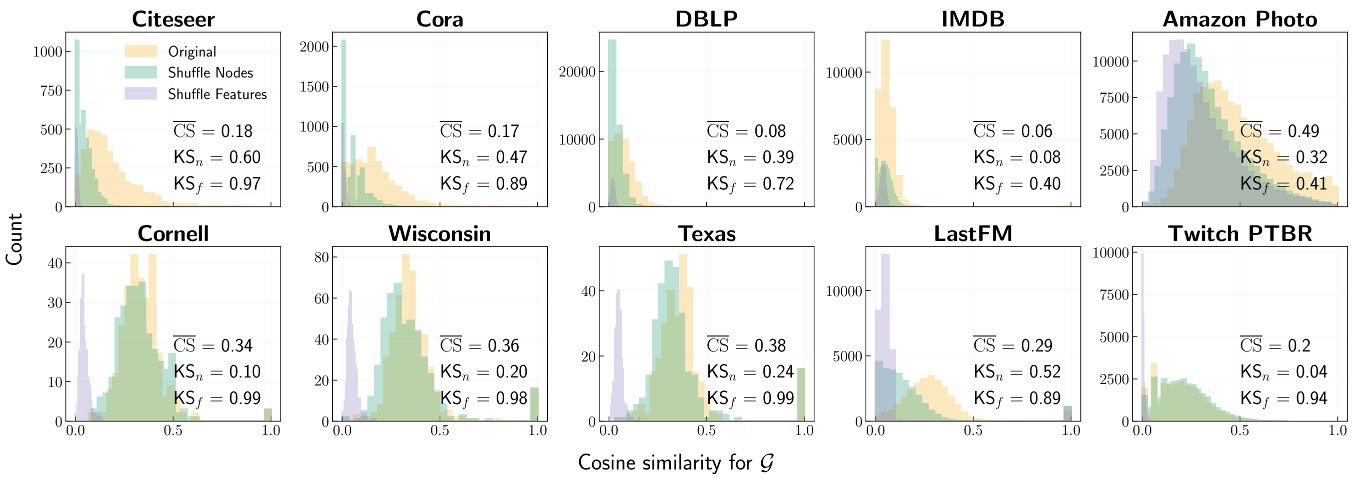


Supplementary Fig. 5: Distribution of the cosine similarities for $\mathcal{G}$. We perform two randomizations: *Shuffle Nodes* – when node features are randomly reassigned and *Shuffle Features* – when the features within a given node feature are shuffled. To assess how (dis)similar are the distributions we ran the Kolmogorov-Smirnov (KS) test. The KS statistic should be a high value (max(KS) = 1) when the fit is good and a low value (min(KS) = 0) when the fit is not good. $\overline{\text{CS}}$ is the average value of cosine similarities.

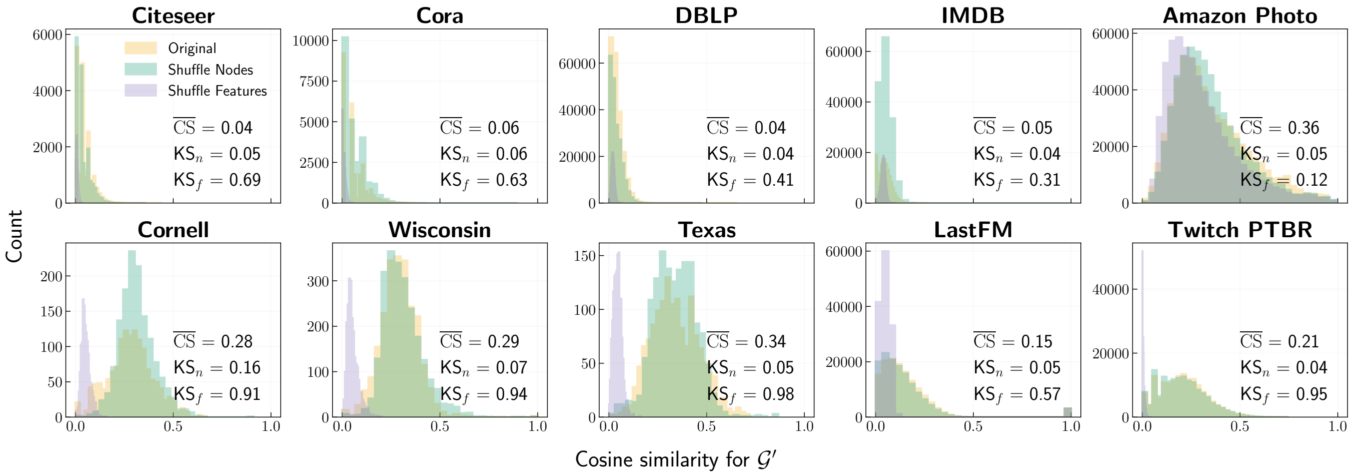


Supplementary Fig. 6: Distribution of the cosine similarities for $\mathcal{G}'$. See caption in Supplementary Fig. 5 for more details.

| | $\overline{\mathrm{CS}}(\mathcal{G})$ | $\sigma(\mathrm{CS}(\mathcal{G}))$ | $\overline{\mathrm{CS}}(\mathcal{G}')$ | $\sigma(\mathrm{CS}(\mathcal{G}'))$ | $\mathrm{corr}(\mathcal{G}, F)$ |
|---|---|---|---|---|---|
| Cora | 0.166 | 0.126 | 0.058 | 0.059 | 0.650 |
| Citeseer | 0.177 | 0.132 | 0.042 | 0.040 | 0.763 |
| IMDB | 0.057 | 0.060 | 0.047 | 0.031 | 0.172 |
| DBLP | 0.075 | 0.053 | 0.037 | 0.033 | 0.506 |
| LastFM | 0.285 | 0.159 | 0.152 | 0.155 | 0.465 |
| Texas | 0.384 | 0.167 | 0.340 | 0.122 | 0.116 |
| Amazon Photo | 0.488 | 0.203 | 0.356 | 0.191 | 0.270 |
| Twitch PTBR | 0.197 | 0.121 | 0.208 | 0.118 | -0.053 |
| Wisconsin | 0.364 | 0.147 | 0.291 | 0.095 | 0.201 |
| Cornell | 0.339 | 0.111 | 0.282 | 0.116 | 0.169 |

Supplementary Table. I: The average and standard deviation of the cosine similarities for $\mathcal{G}$ and $\mathcal{G}'$. The last column shows the relative difference between the average cosine similarities.

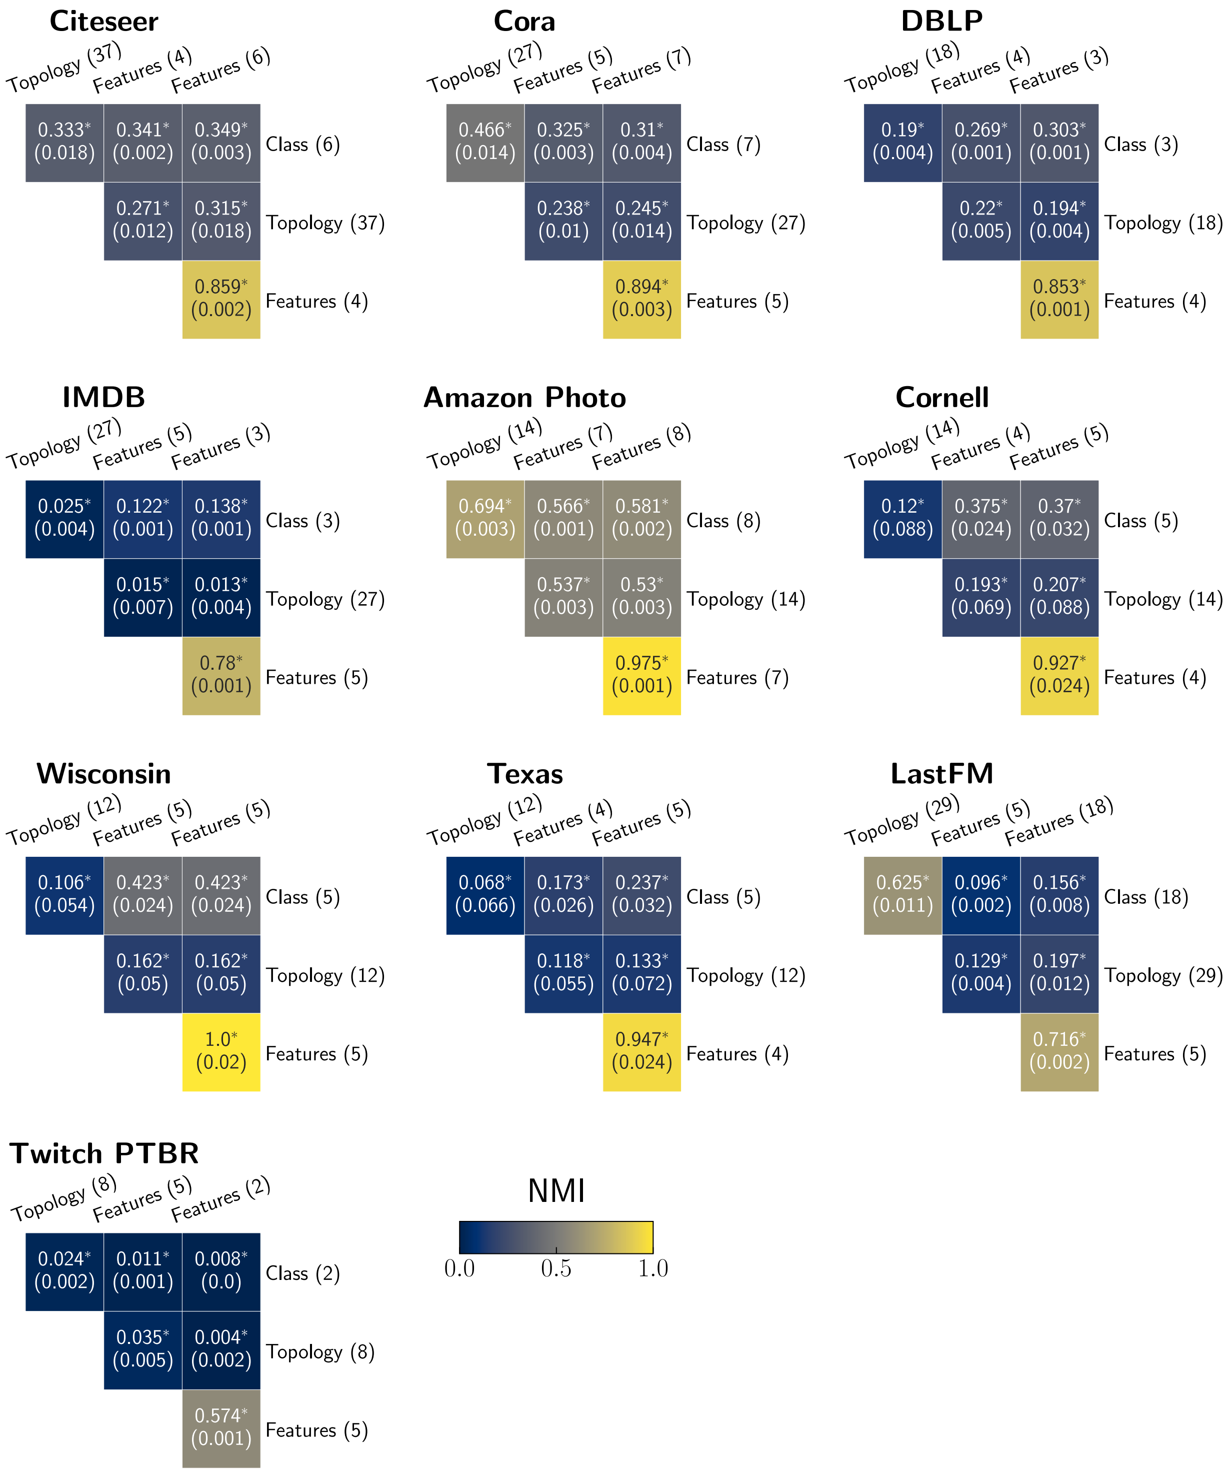


Supplementary Fig. 7: Normalized mutual information (NMI) between each of two different sets of labels. The randomized version of NMI is shown in the brackets as the second row in each entry. That value is averaged over 100 random shufflings. The number displayed next to the label type indicates the number of classes. There are two cases for feature-based labels: (i) when the number of classes is obtained using the community concentration measure or (ii) the number of classes is set as in the metadata.

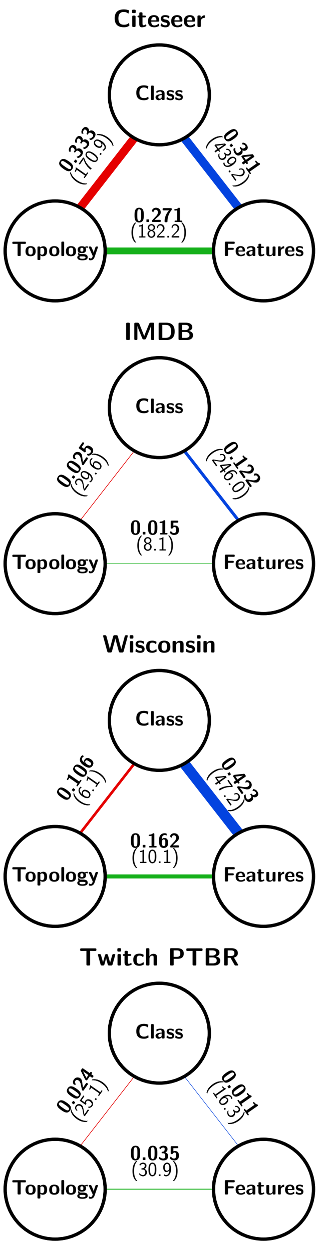


Supplementary Fig. 8: Normalized mutual information (NMI) between each of two different sets of labels. The value in bracket represents the z-score (see main text). The width of the line is proportional to NMI.

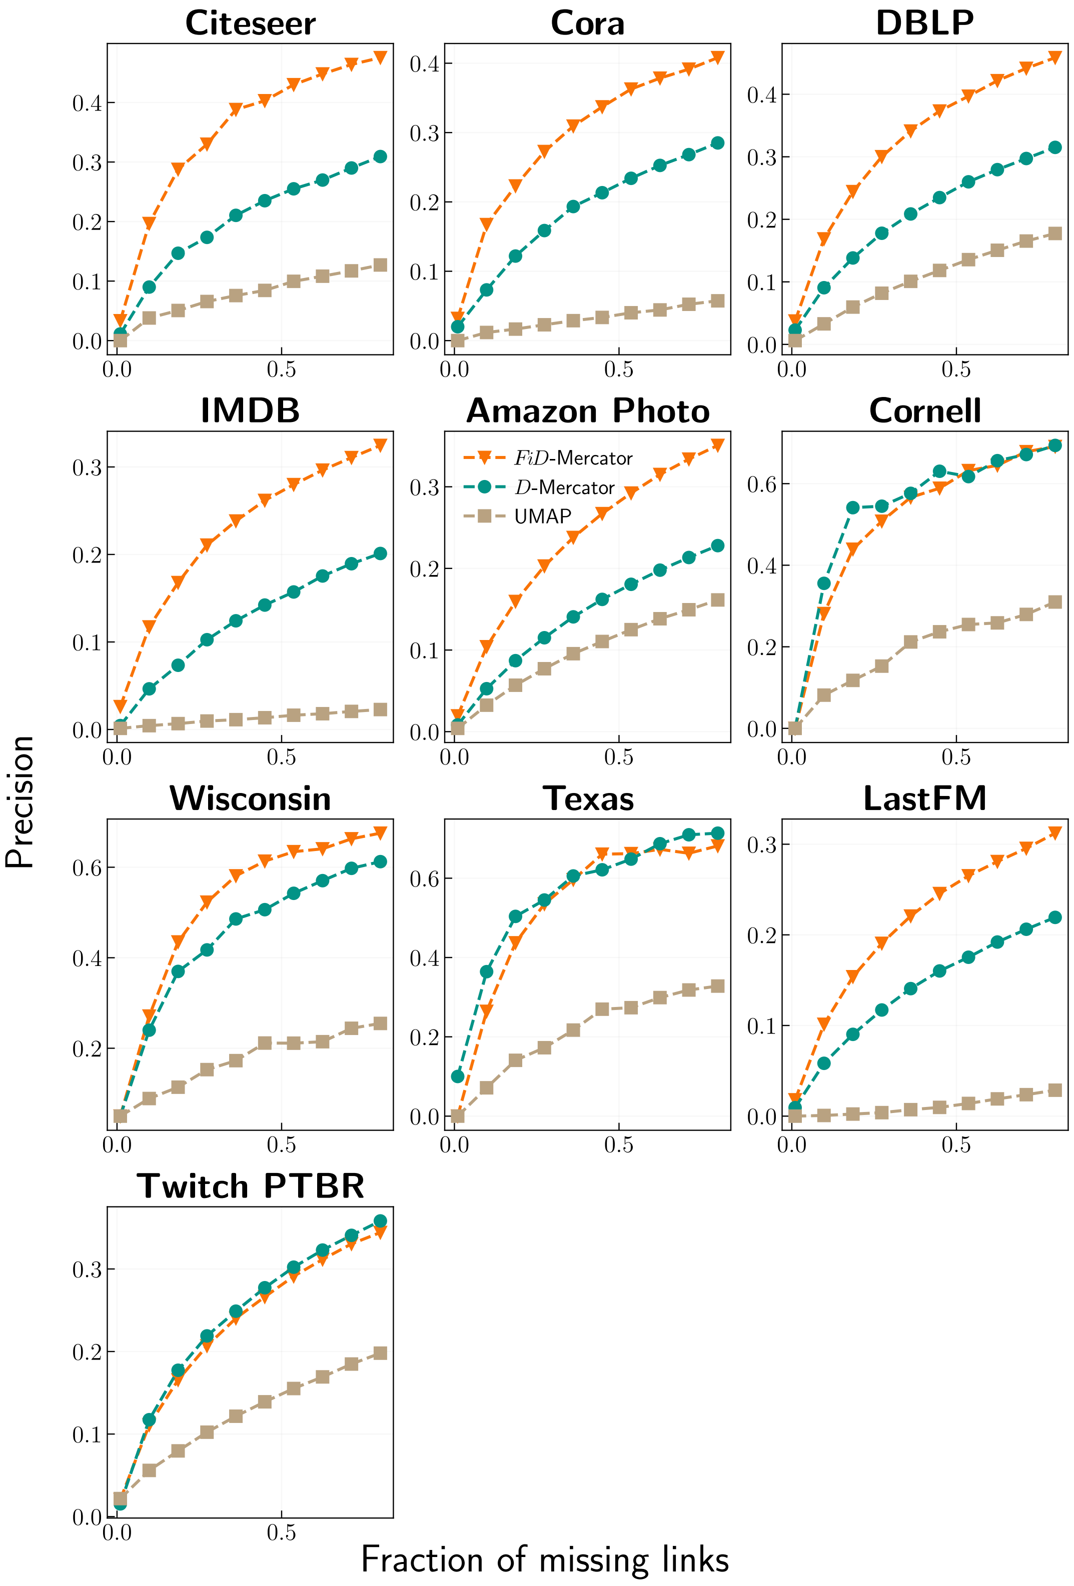


Supplementary Fig. 9: Precision as the function of the fraction of missing links for link prediction task. The results are averaged over five realizations.

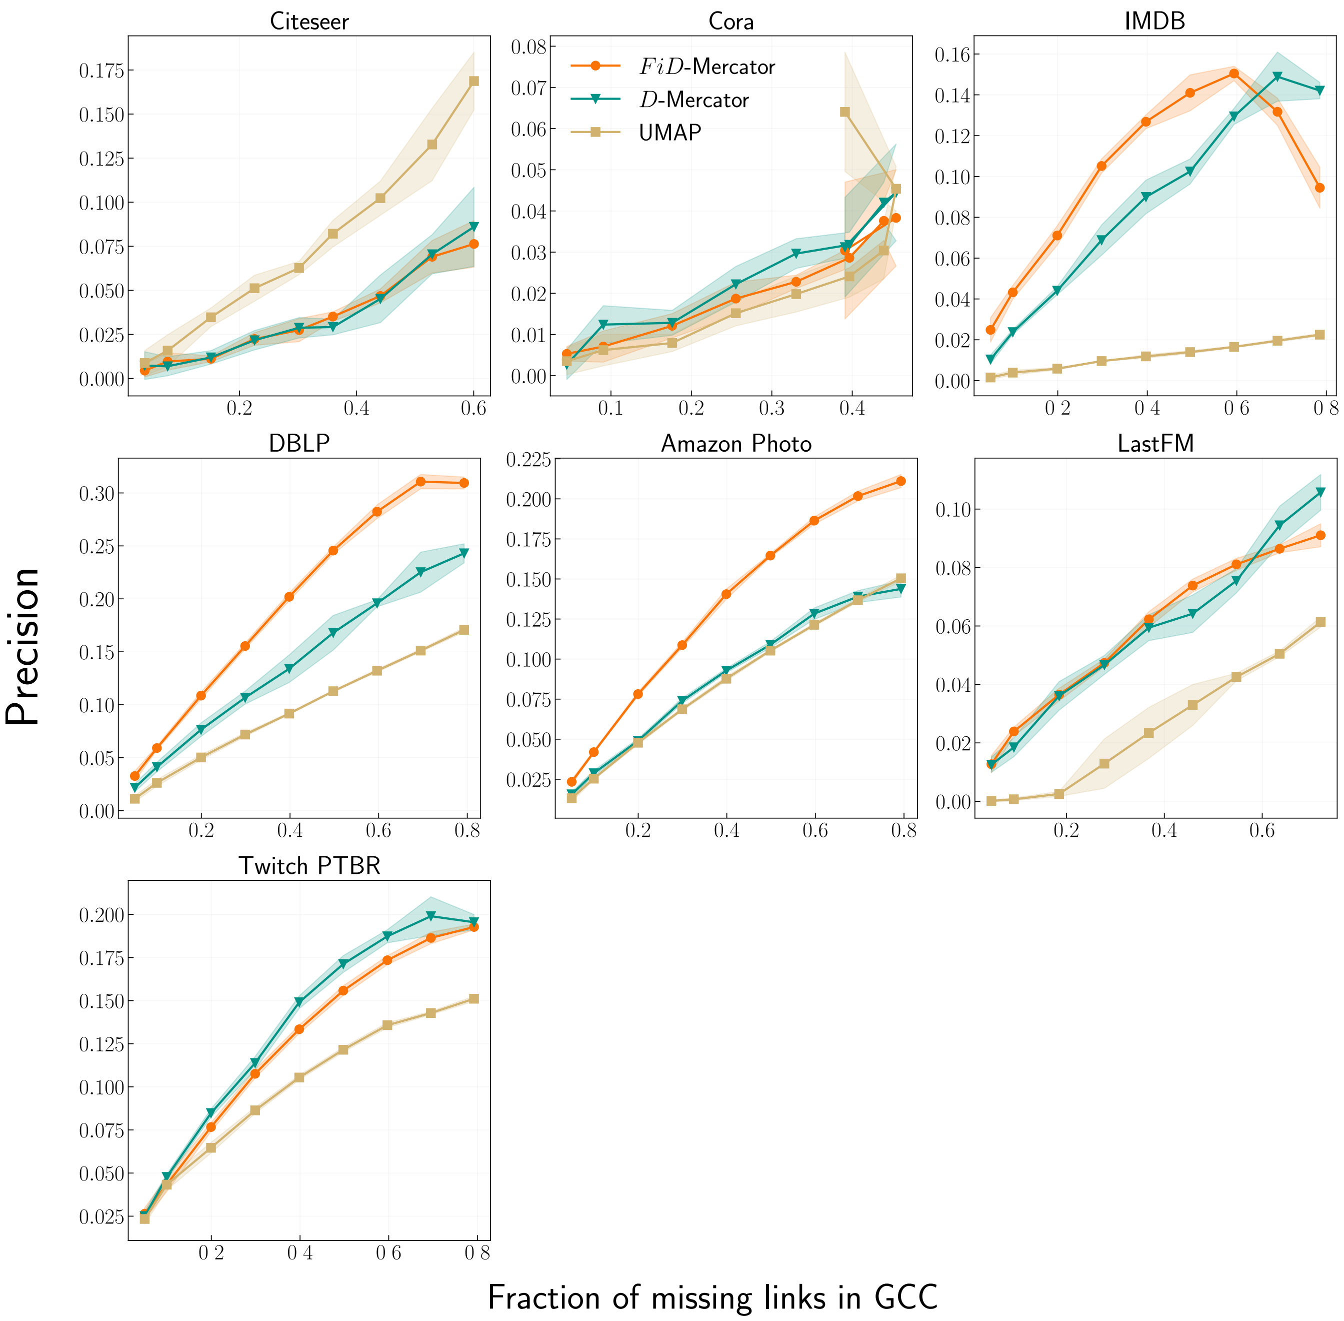


Supplementary Fig. 10: Precision as the function of the fraction of missing links in GCC for link prediction task. We omitted the Cornell, Wisconsin, and Texas networks due to their small size after the removal of a large fraction of links. The results are averaged over five realizations.

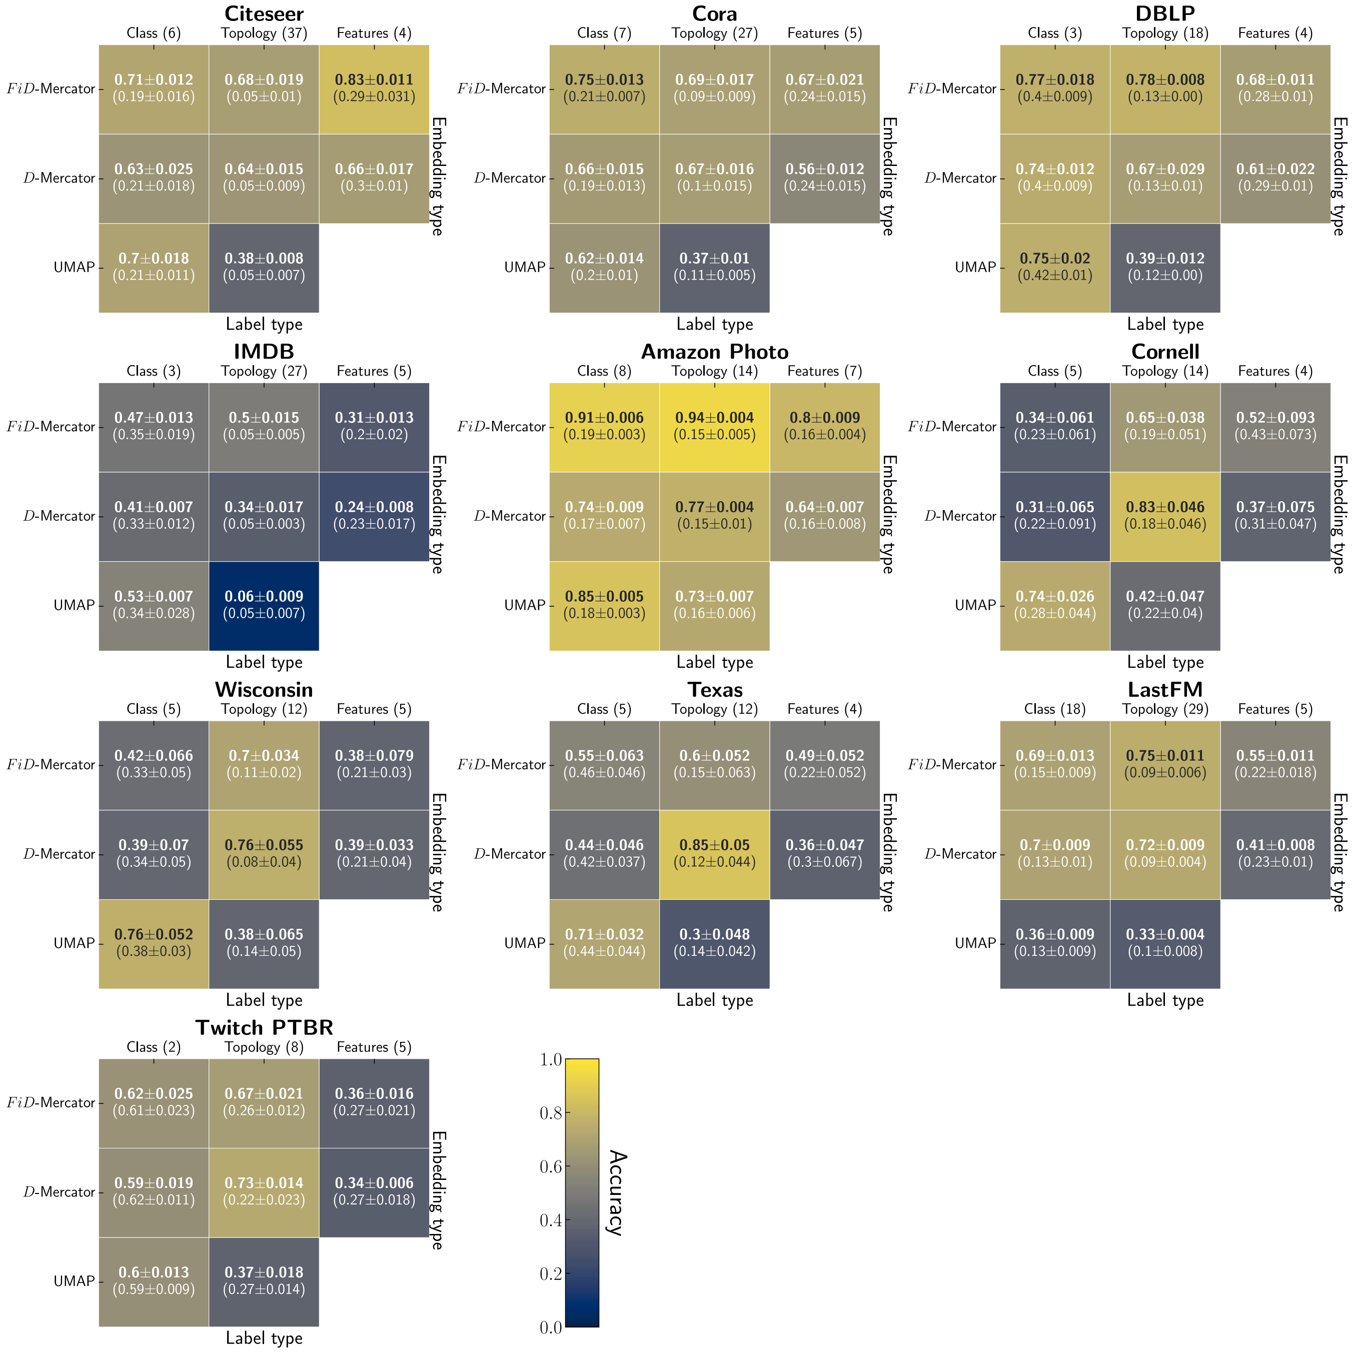


Supplementary Fig. 11: Accuracy heatmaps of node classification task. Each row represents a different embedding method, whereas each column a different set of labels. In brackets, the number of labels is shown. The performance of node classification on shuffled labels is displayed in brackets as the second row in each entry. Train-test size split: 80/20. Results are averaged over five different train-test splits.

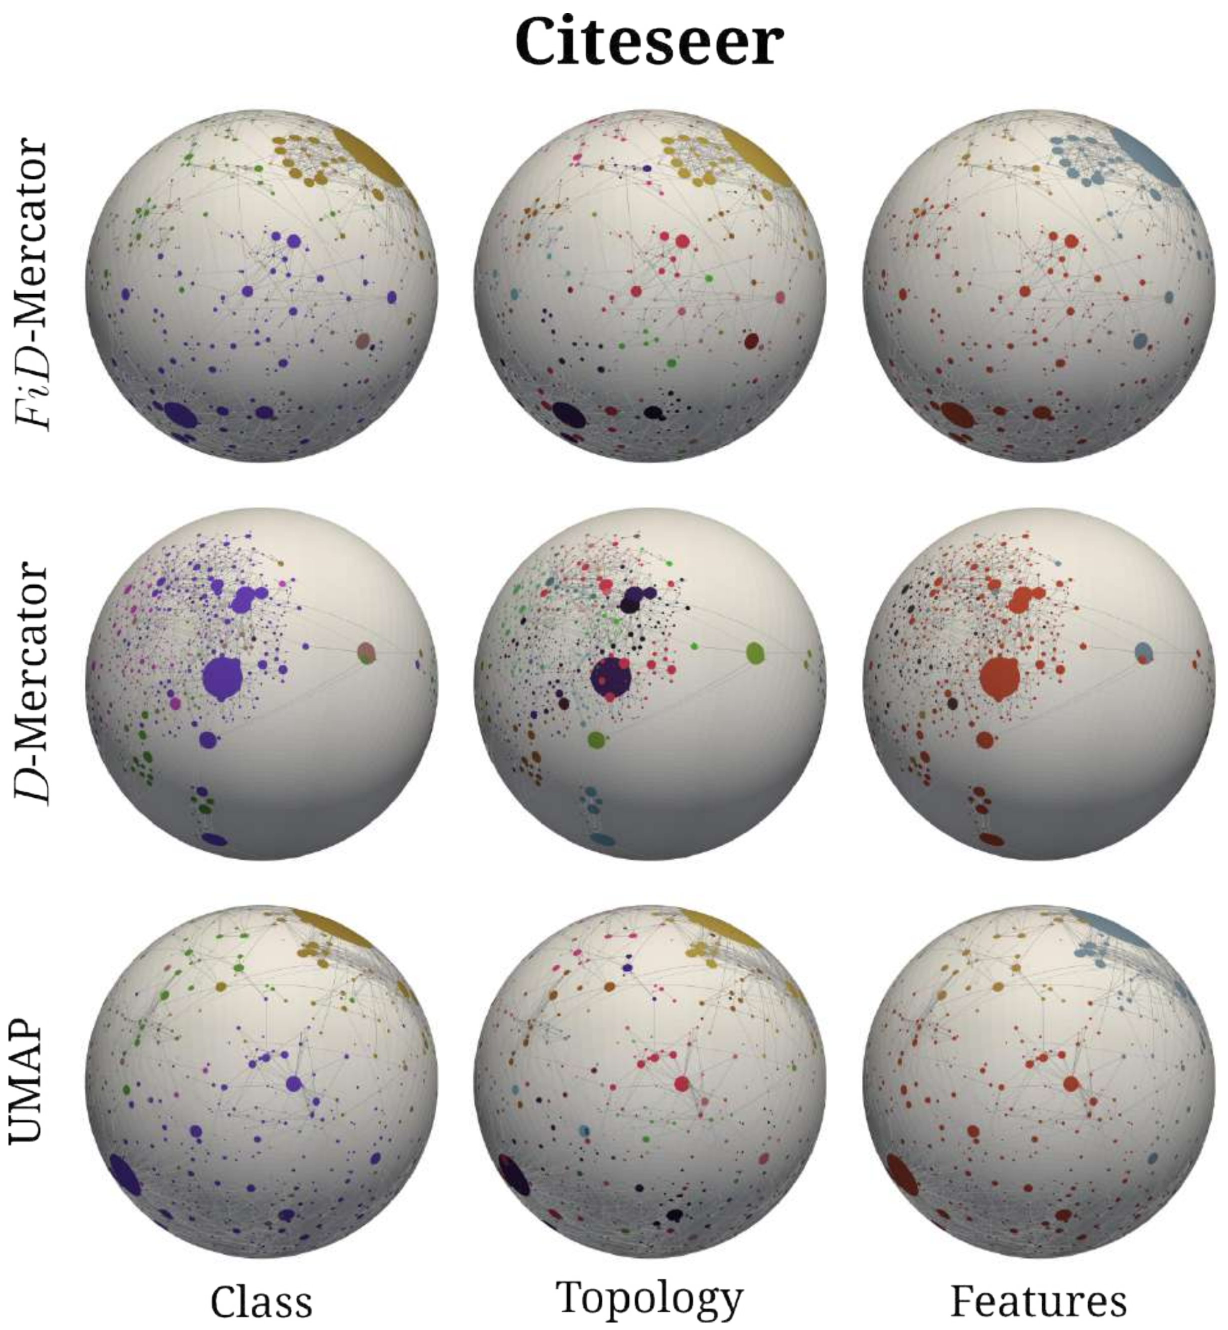


Supplementary Fig. 12: The panels show the embeddings of the Citeseer network. Each row corresponds to the different embedding method whereas each columns to different assignment of labels. The size of a node is proportional to its expected degree, and its color indicates the community it belongs to. For the sake of clarity, only the connections with probability $p_{ij} > 0.5$ are shown.

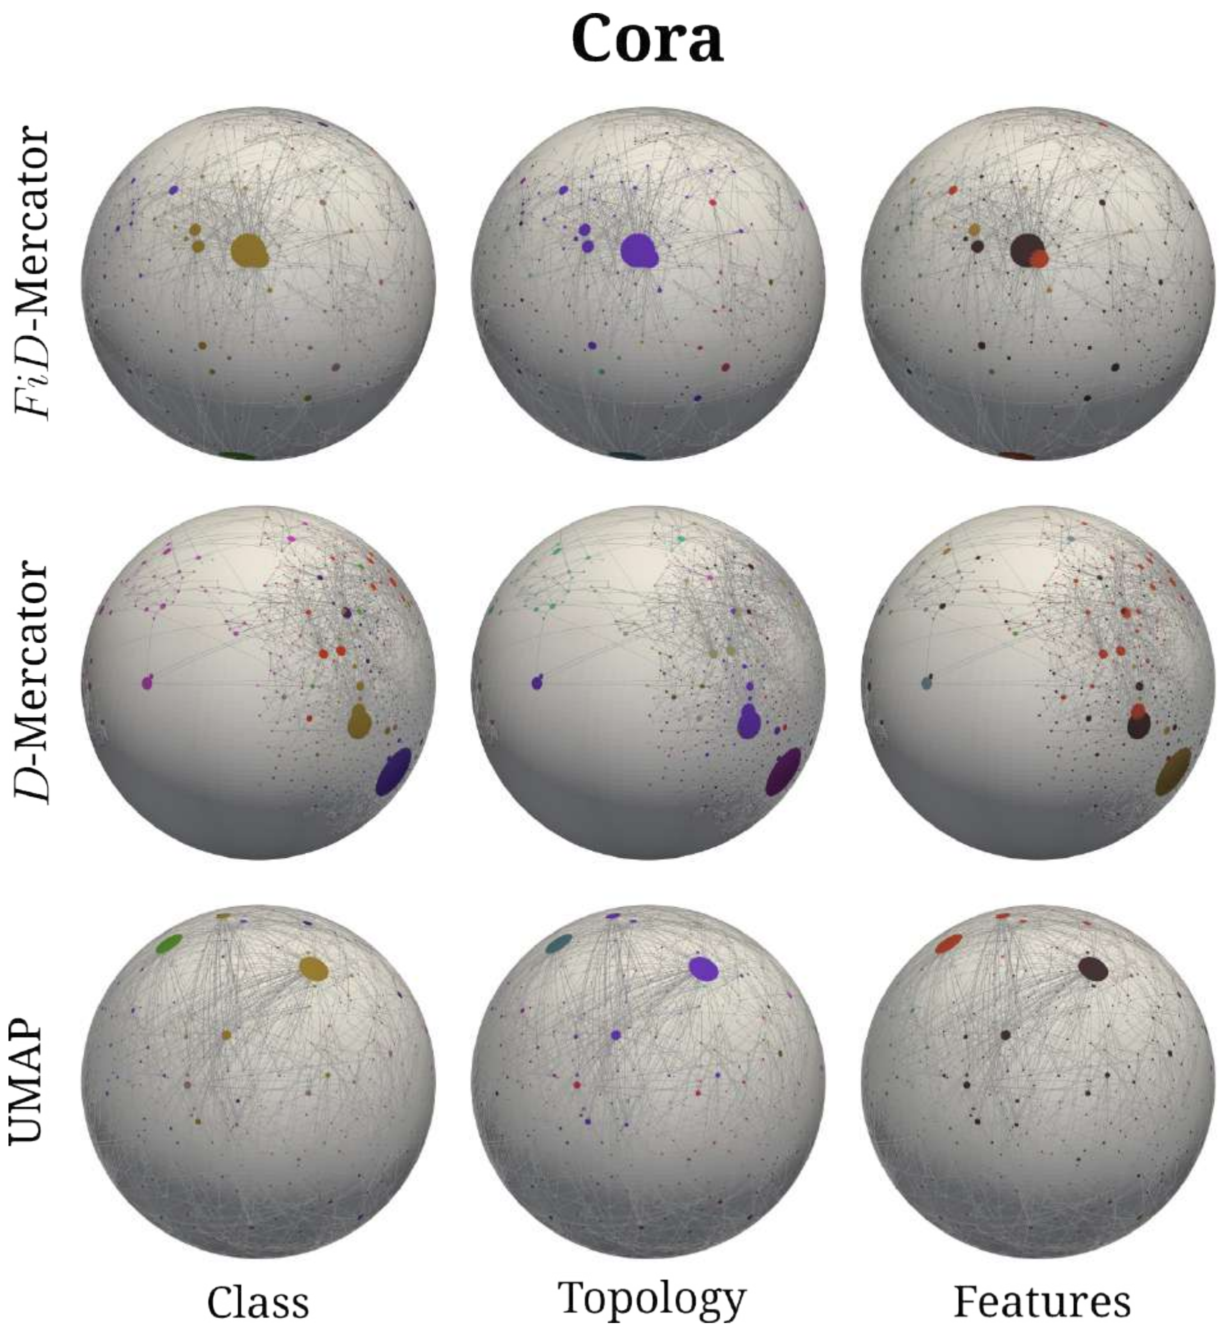


Supplementary Fig. 13: The panels show the embeddings of the Cora network. For more details see Supplementary Fig. 12. For the sake of clarity, only the connections with probability $p_{ij} > 0.5$ are shown.

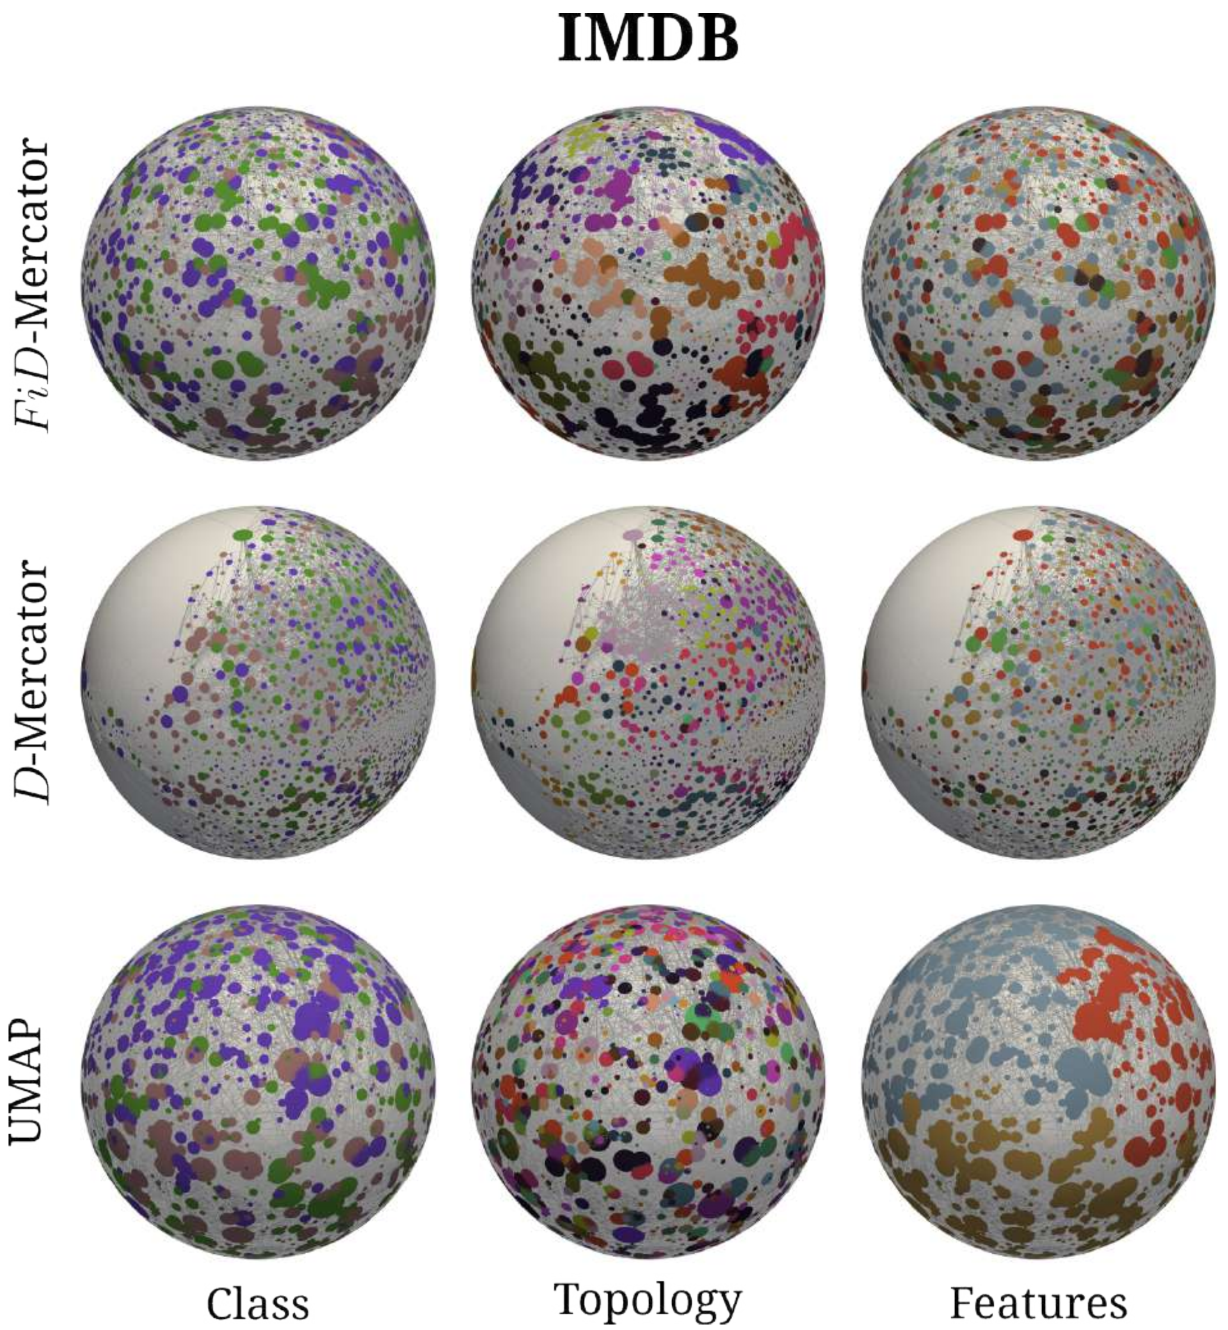


Supplementary Fig. 14: The panels show the embeddings of the IMDB network. For more details see Supplementary Fig. 12. For the sake of clarity, only the connections with probability $p_{ij} > 0.999$ are shown.

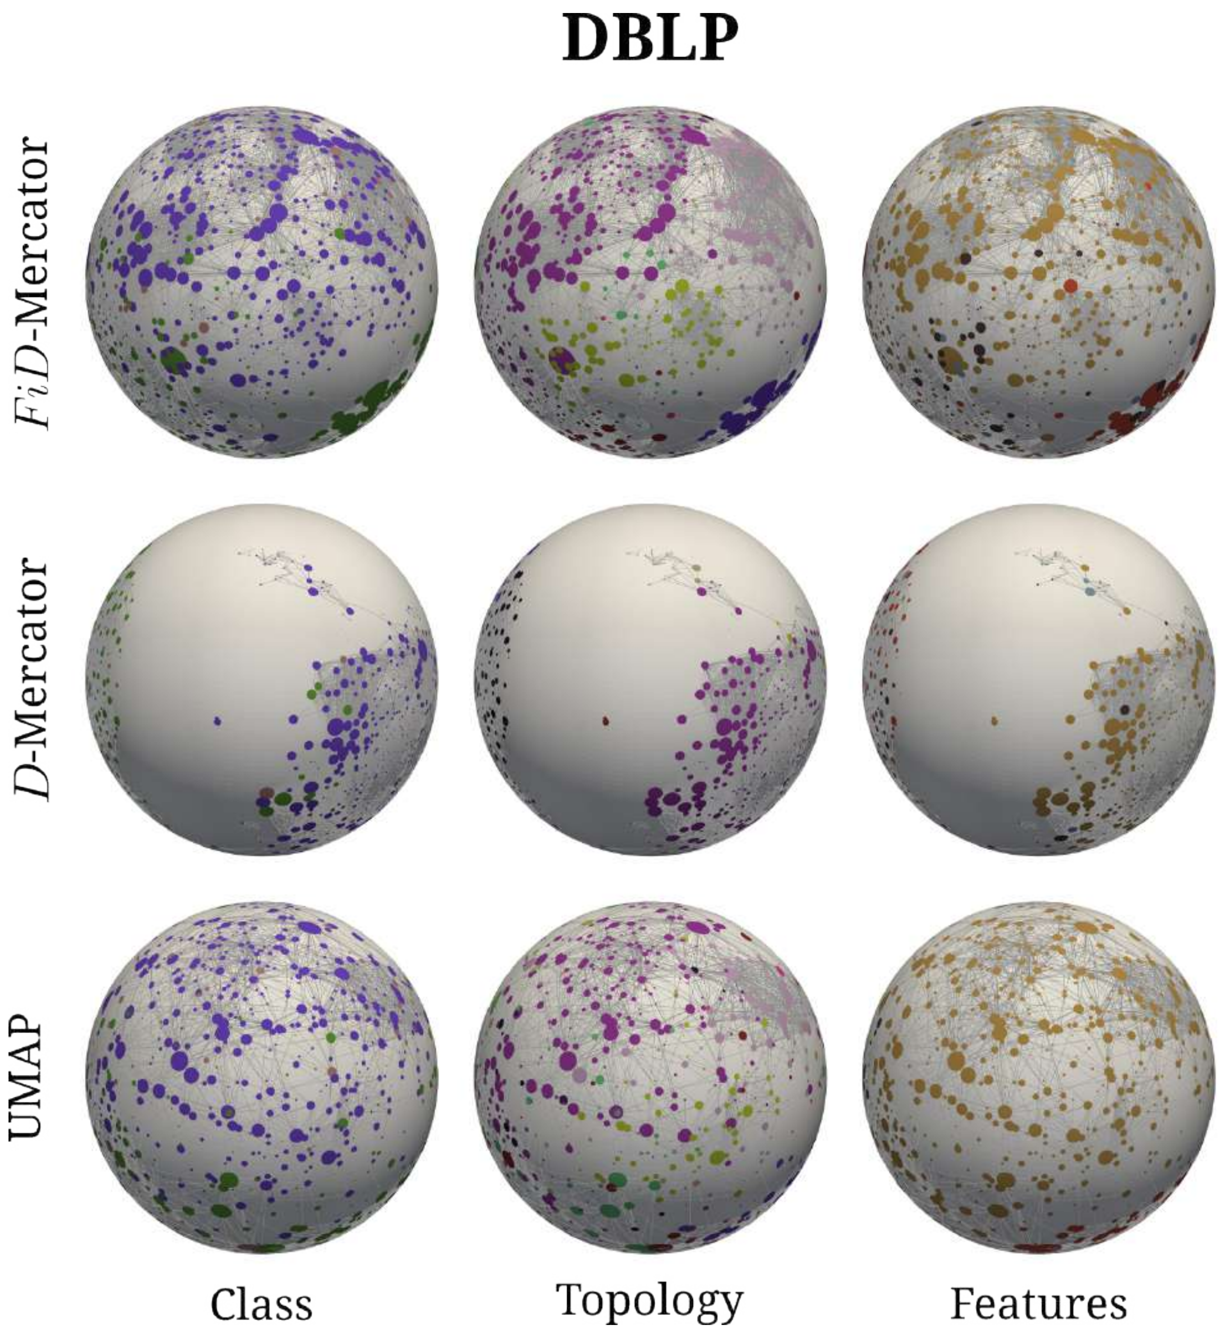


Supplementary Fig. 15: The panels show the embeddings of the IMDB network. For more details see Supplementary Fig. 12. For the sake of clarity, only the connections with probability $p_{ij} > 0.99999$ are shown.

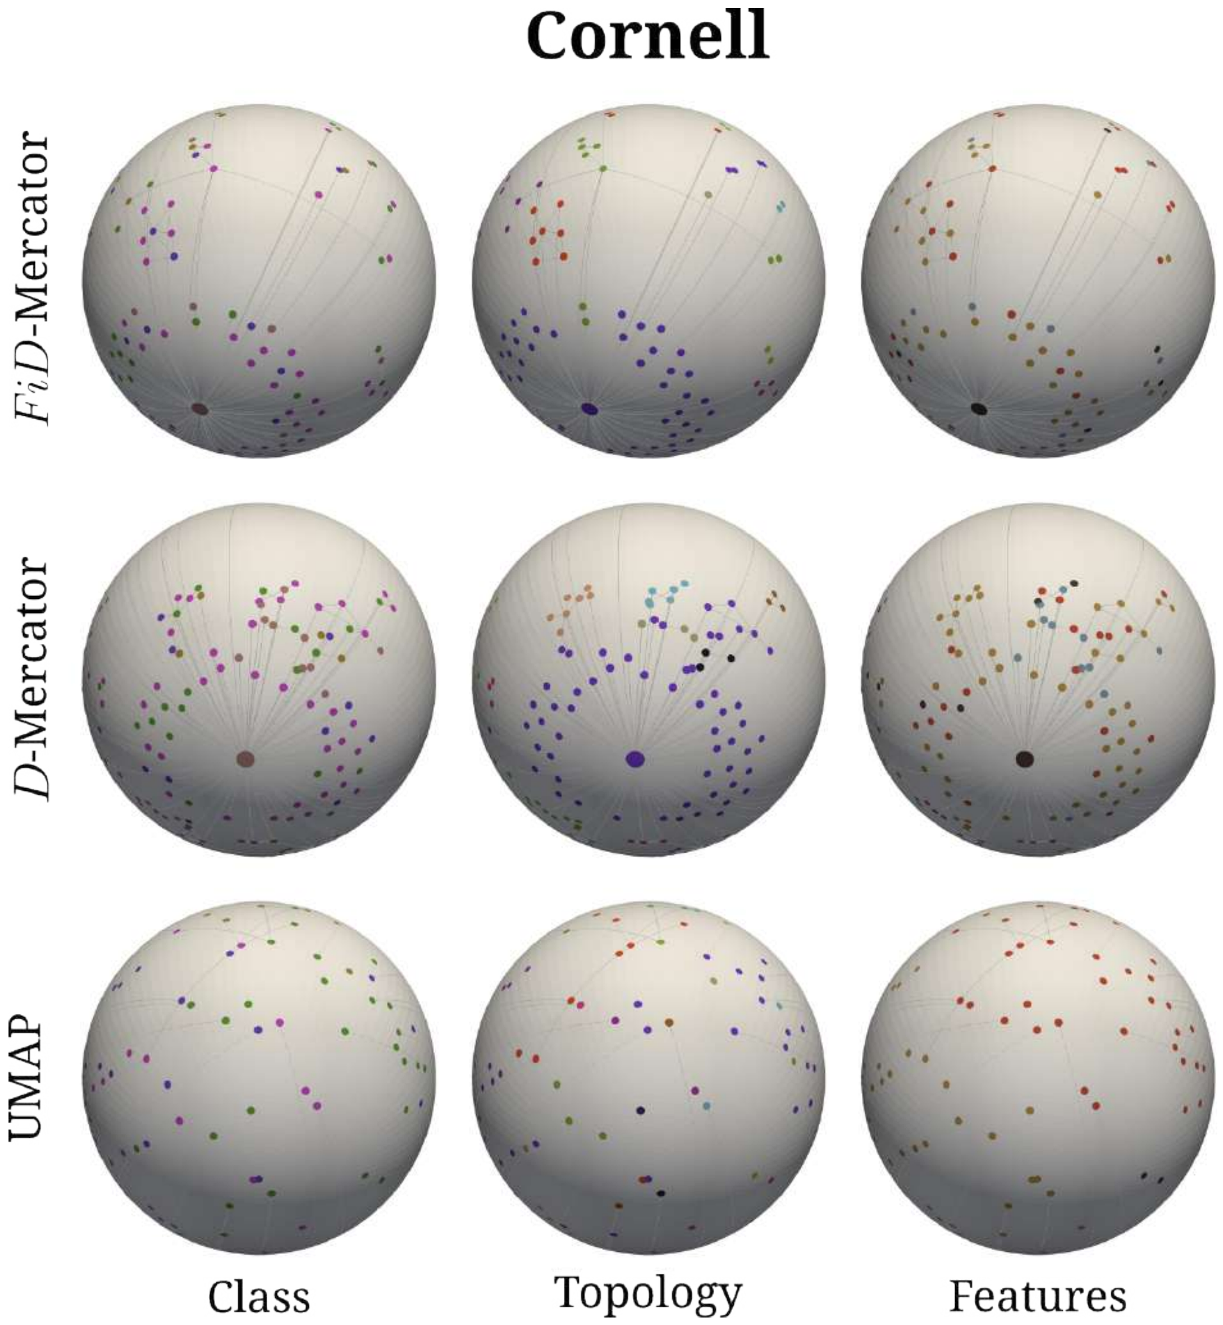


Supplementary Fig. 16: The panels show the embeddings of the Cornell network. For more details see Supplementary Fig. 12. For the sake of clarity, only the connections with probability $p_{ij} > 0.5$ are shown.

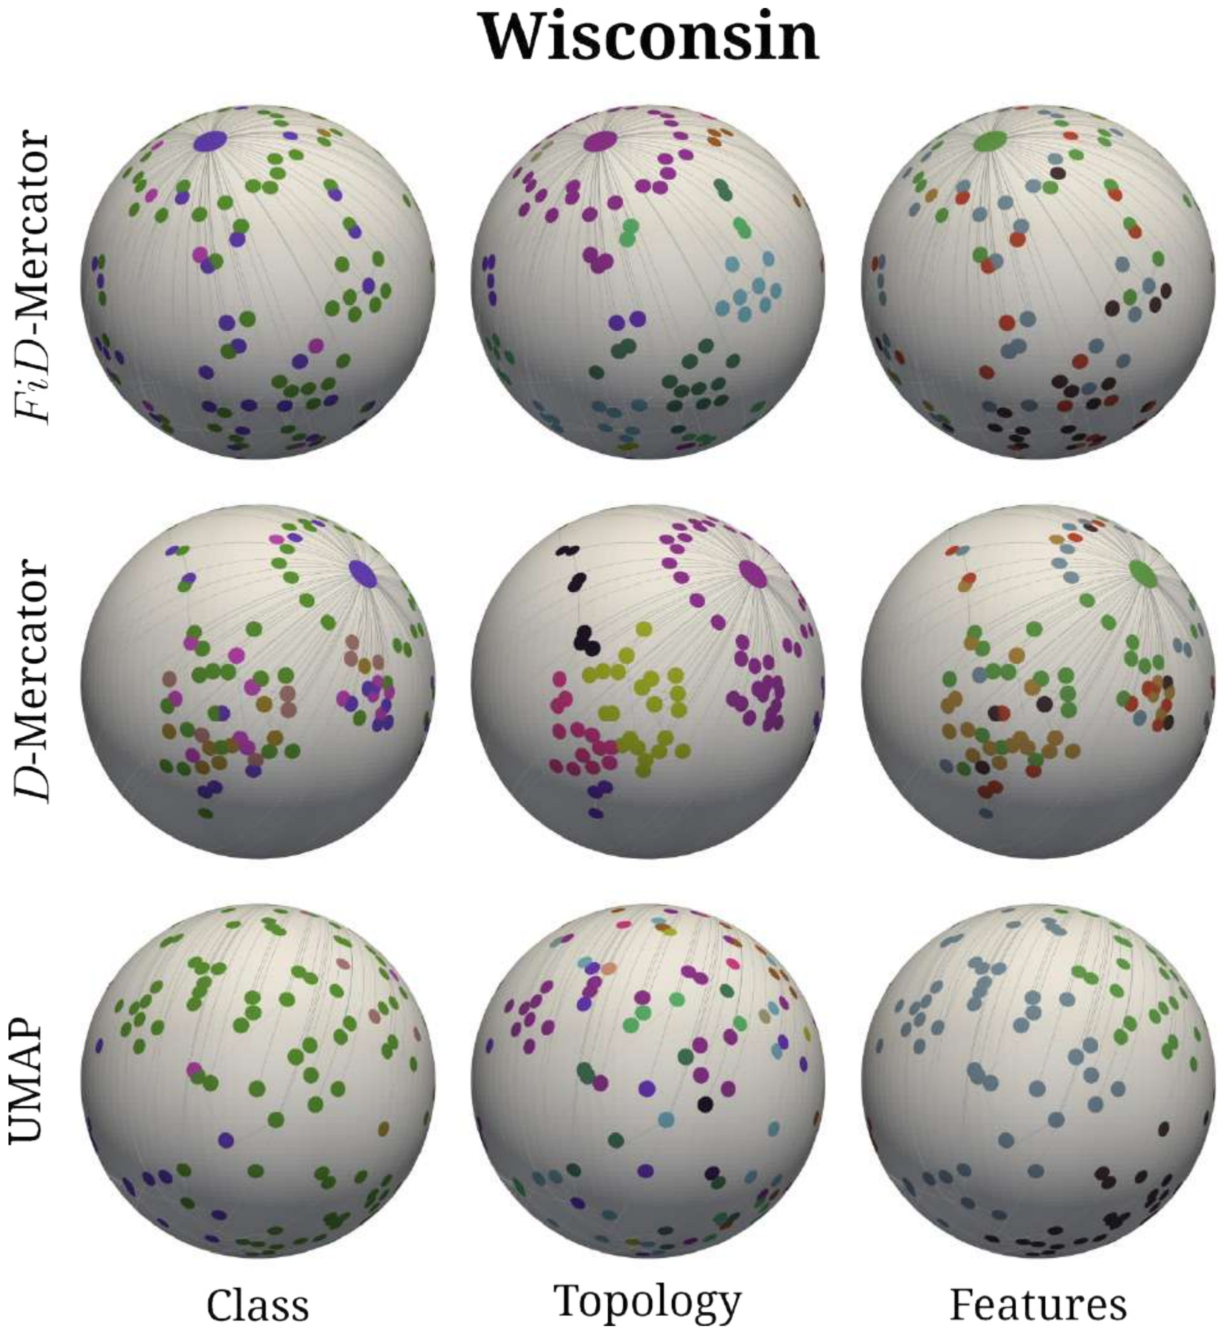


Supplementary Fig. 17: The panels show the embeddings of the Wisconsin network. For more details see Supplementary Fig. 12. For the sake of clarity, only the connections with probability $p_{ij} > 0.5$ are shown.

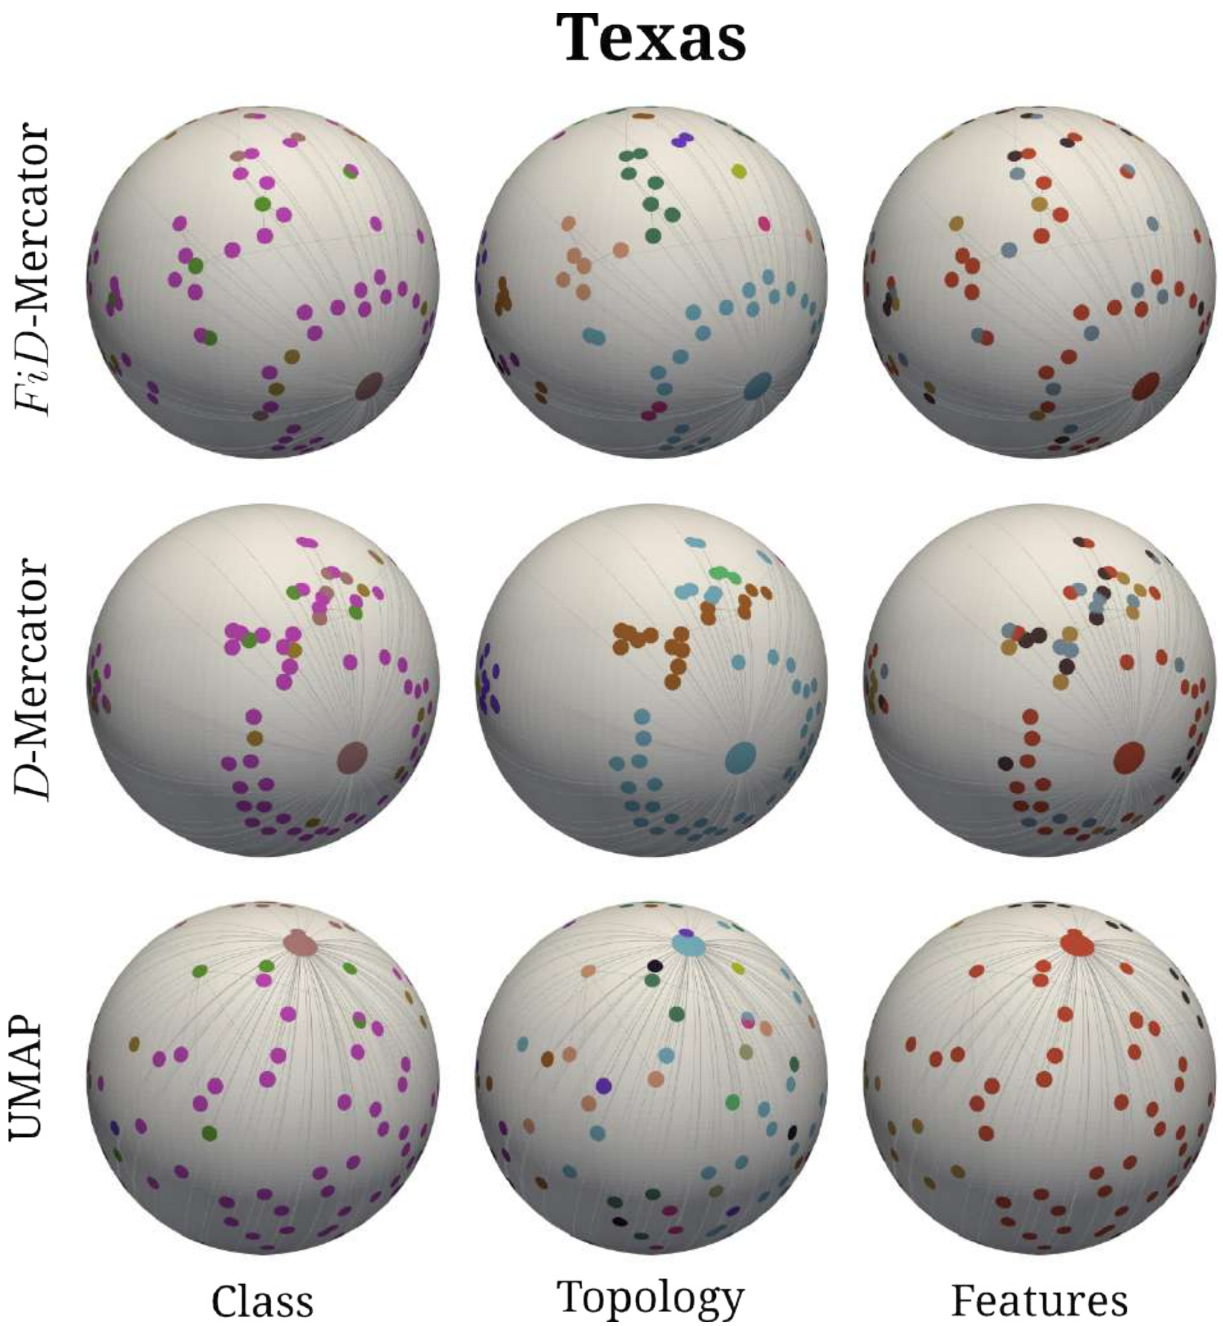


Supplementary Fig. 18: The panels show the embeddings of the Texas network. For more details see Supplementary Fig. 12. For the sake of clarity, only the connections with probability $p_{ij} > 0.5$ are shown.

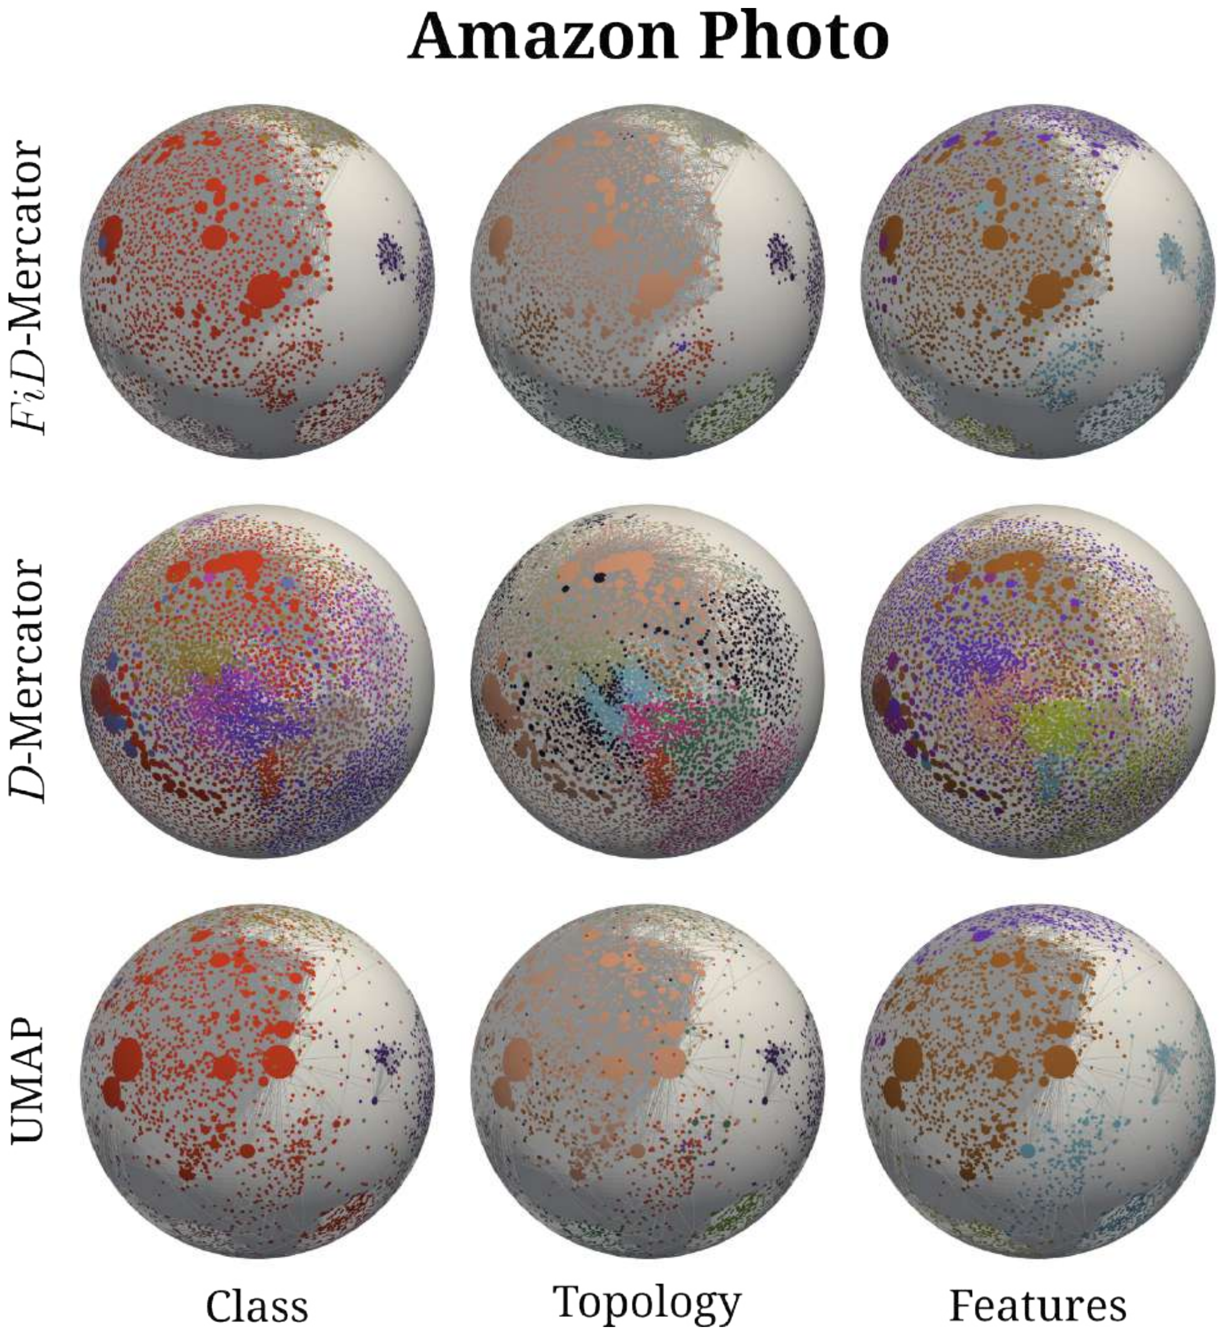


Supplementary Fig. 19: The panels show the embeddings of the Amazon Photo network. For more details see Supplementary Fig. 12. For the sake of clarity, only the connections with probability $p_{ij} > 0.99996$ are shown.

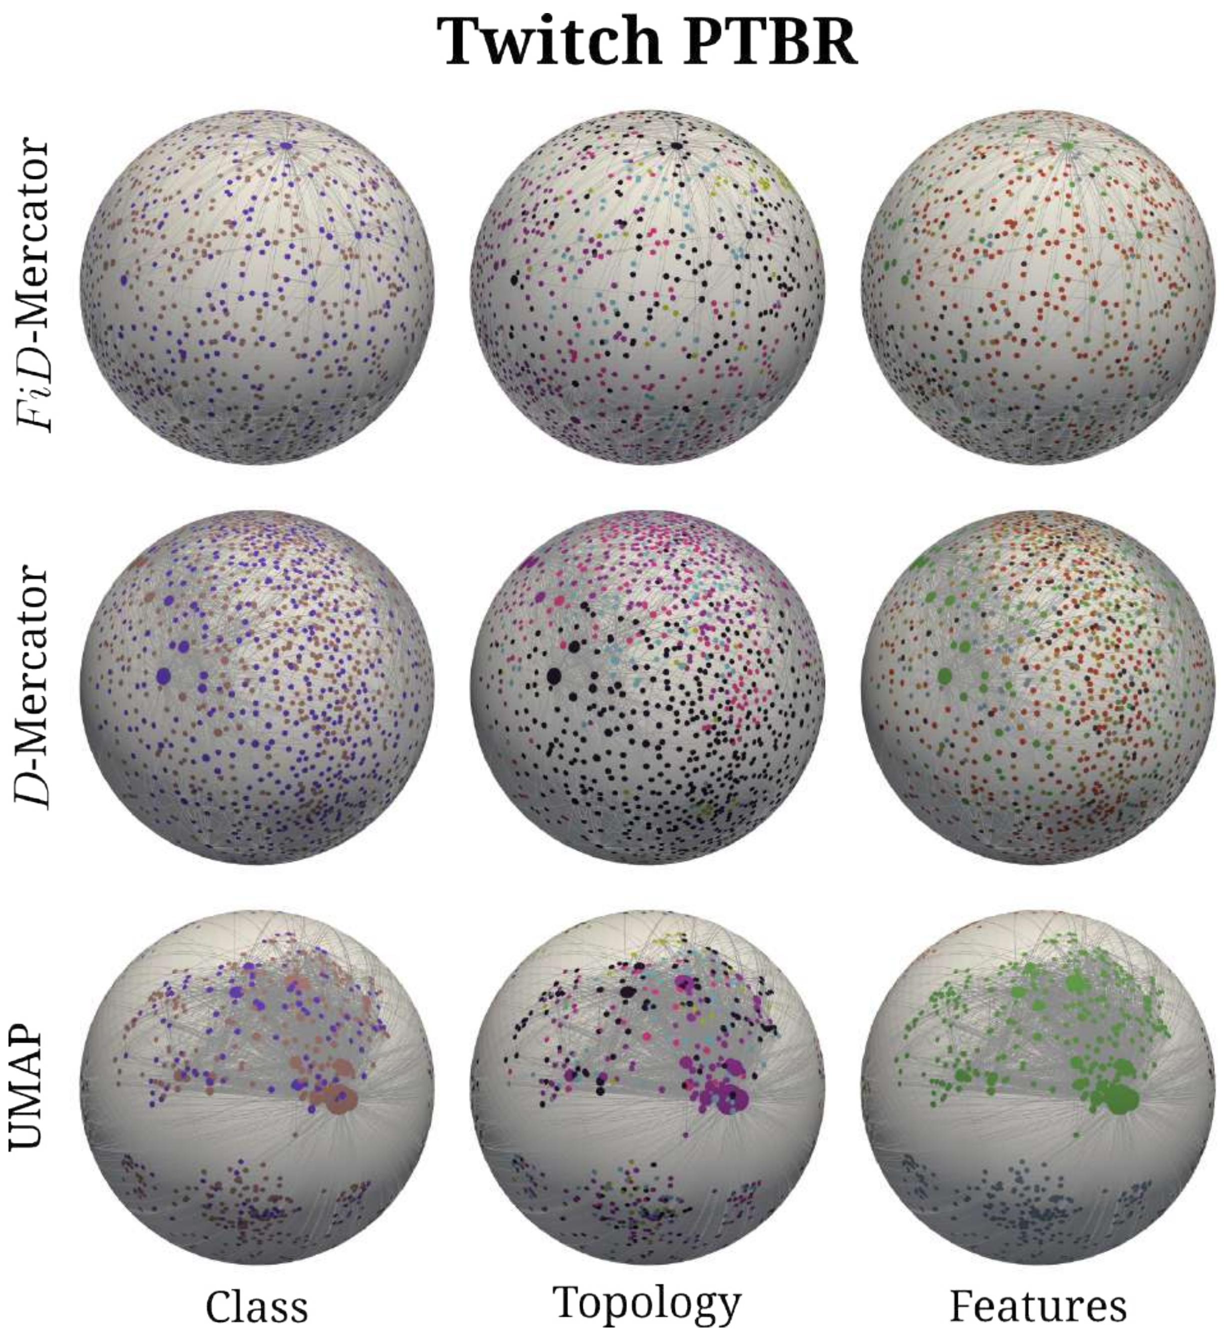


Supplementary Fig. 20: The panels show the embeddings of the Twitch PTBR network. For more details see Supplementary Fig. 12. For the sake of clarity, only the connections with probability $p_{ij} > 0.999$ are shown.

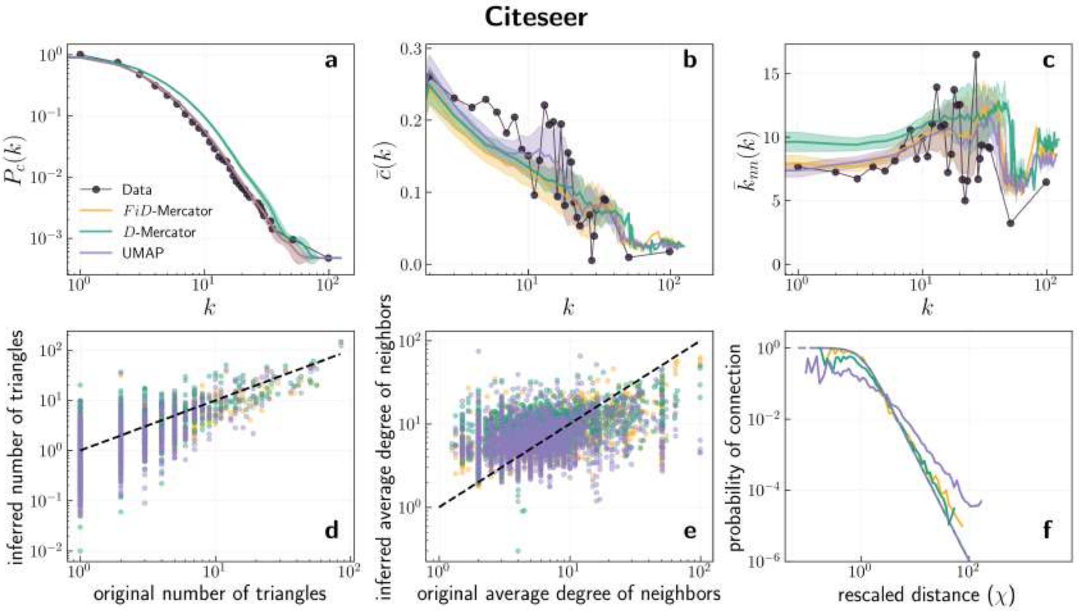


Supplementary Fig. 21: Topological validation of the embeddings of the Citeseer network. Panel (**a**) shows the complementary cumulative degree distribution and panel (**b**) the clustering spectrum $\bar{c}(k)$. Symbols correspond to the value of these quantities in the original network, whereas the lines indicate an estimate of their expected values in the ensemble of random networks in different types of embedding. This ensemble was sampled by generating 100 synthetic networks with the $\mathbb{S}^2$ model and the inferred parameters and positions by $FiD$-Mercator, $D$-Mercator or UMAP. The error bars show the $2\sigma$ confidence interval around the expected value. Panel (**c**) shows the average nearest neighbors degree $\bar{k}_{nn}(k)$. Panels (**d**) and (**e**) depict the scattered plots of the sum of the degrees of their neighbors and the number of triangles in which they participate, respectively. The plots show the estimated values of these two measures in the same ensemble of random networks considered above versus the corresponding values in the original network. Panel (**f**) shows the comparison of the expected connection probability based on the inferred value of $\beta$ (expected) and the actual connection probability computed with the inferred hidden variables.

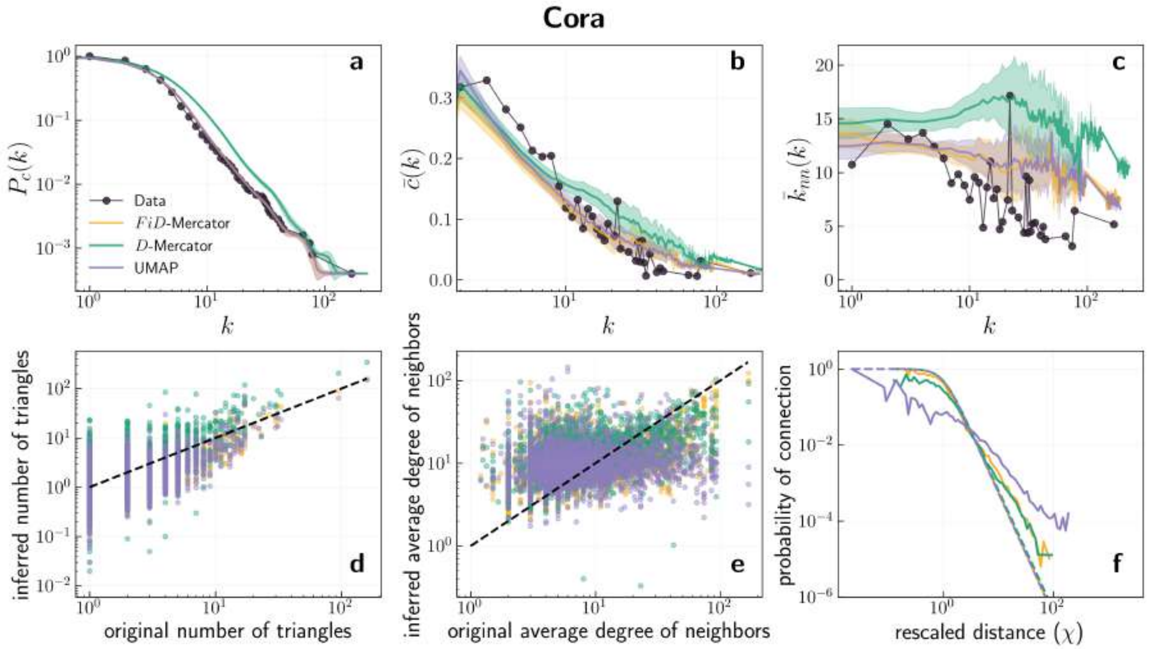


Supplementary Fig. 22: Topological validation of the embeddings of the Cora network. See caption in Supplementary Fig. 21 for more details.

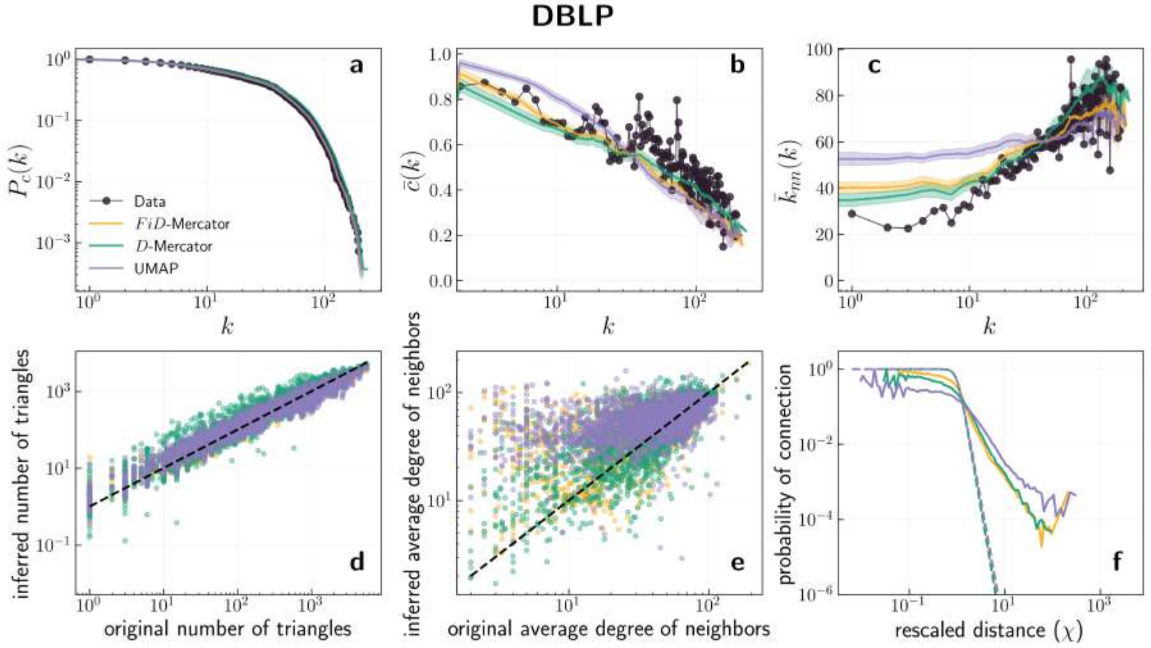


Supplementary Fig. 23: Topological validation of the embeddings of the DBLP network. See caption in Supplementary Fig. 21 for more details.

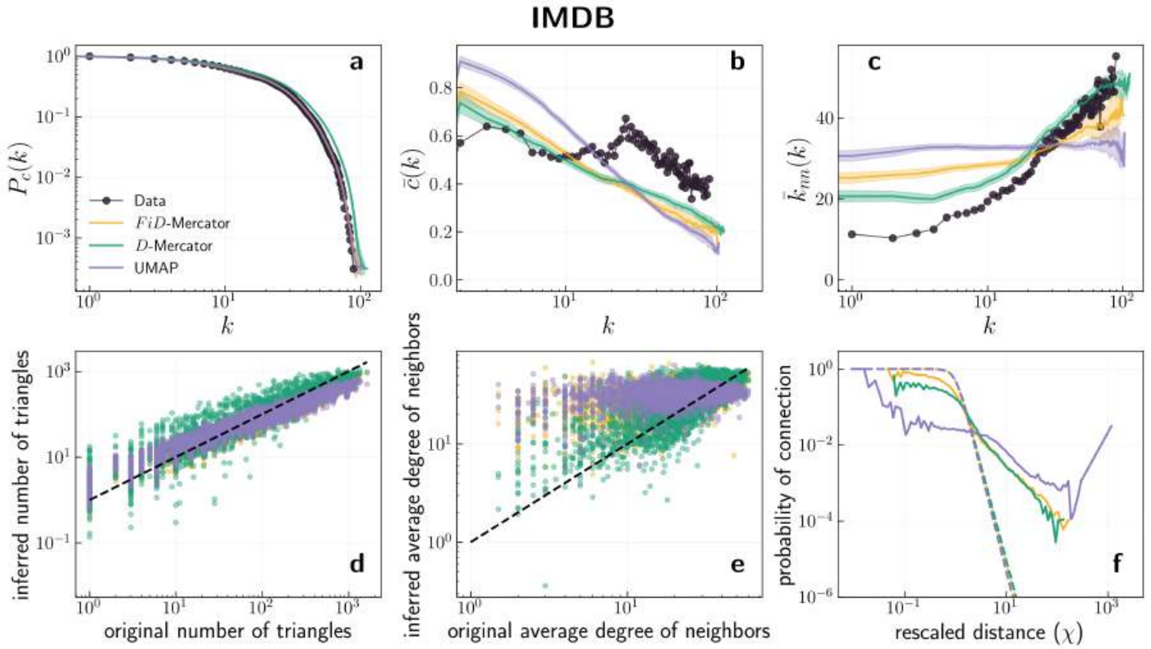


Supplementary Fig. 24: Topological validation of the embeddings of the IMDB network. See caption in Supplementary Fig. 21 for more details.

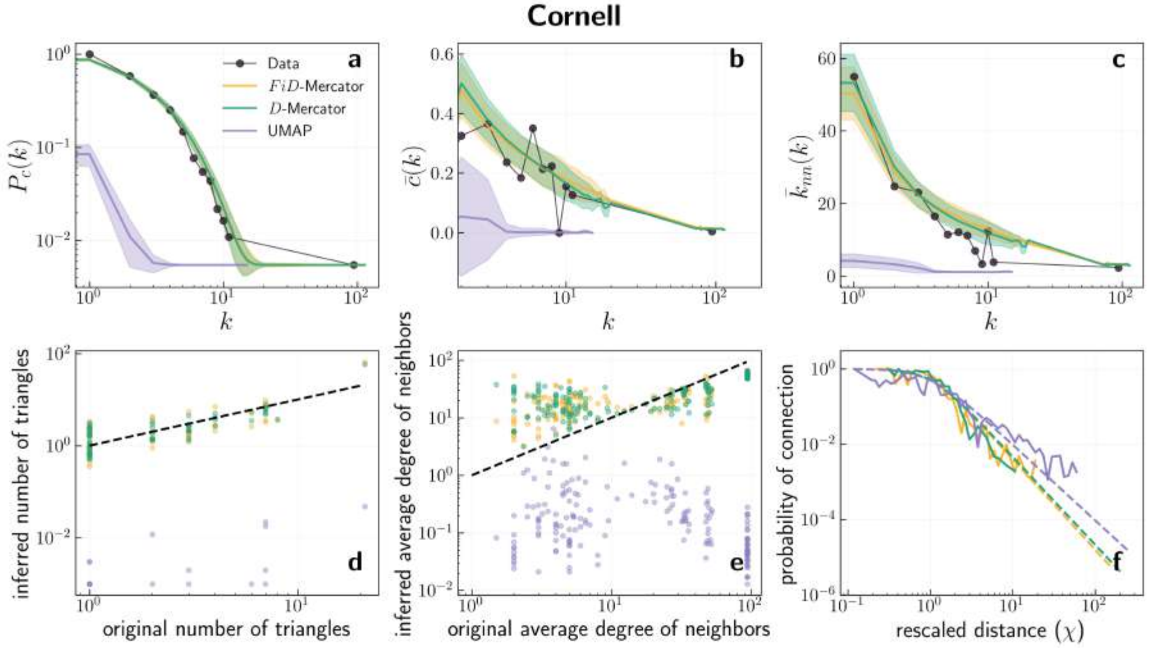


Supplementary Fig. 25: Topological validation of the embeddings of the Cornell network. See caption in Supplementary Fig. 21 for more details.

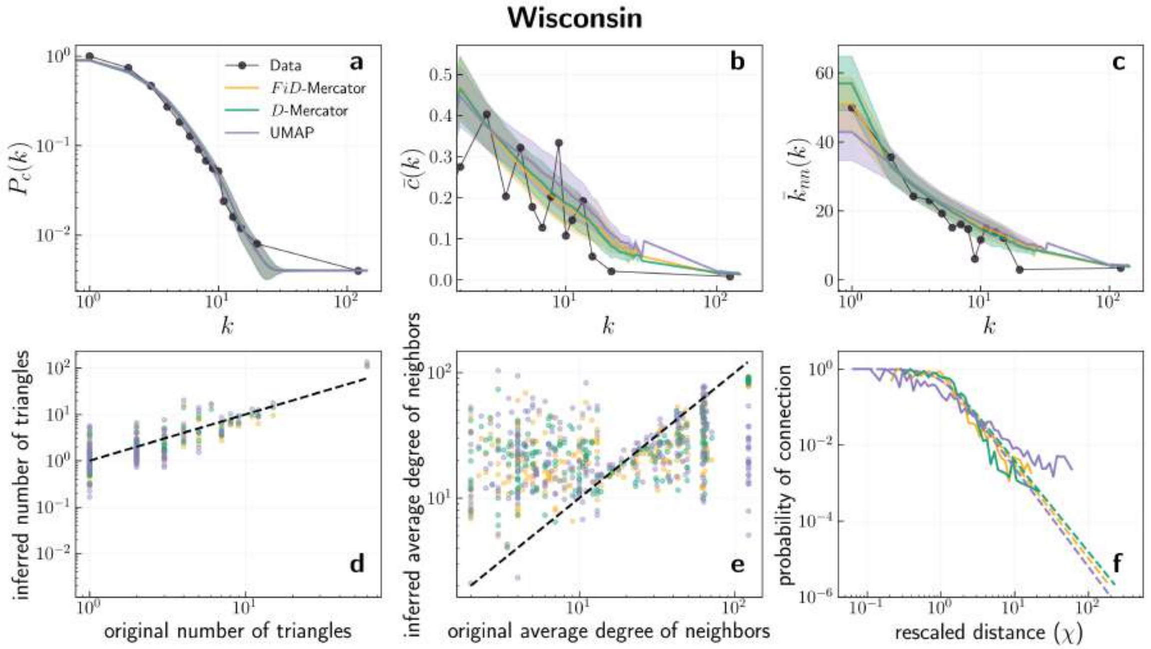


Supplementary Fig. 26: Topological validation of the embeddings of the Wisconsin network. See caption in Supplementary Fig. 21 for more details.

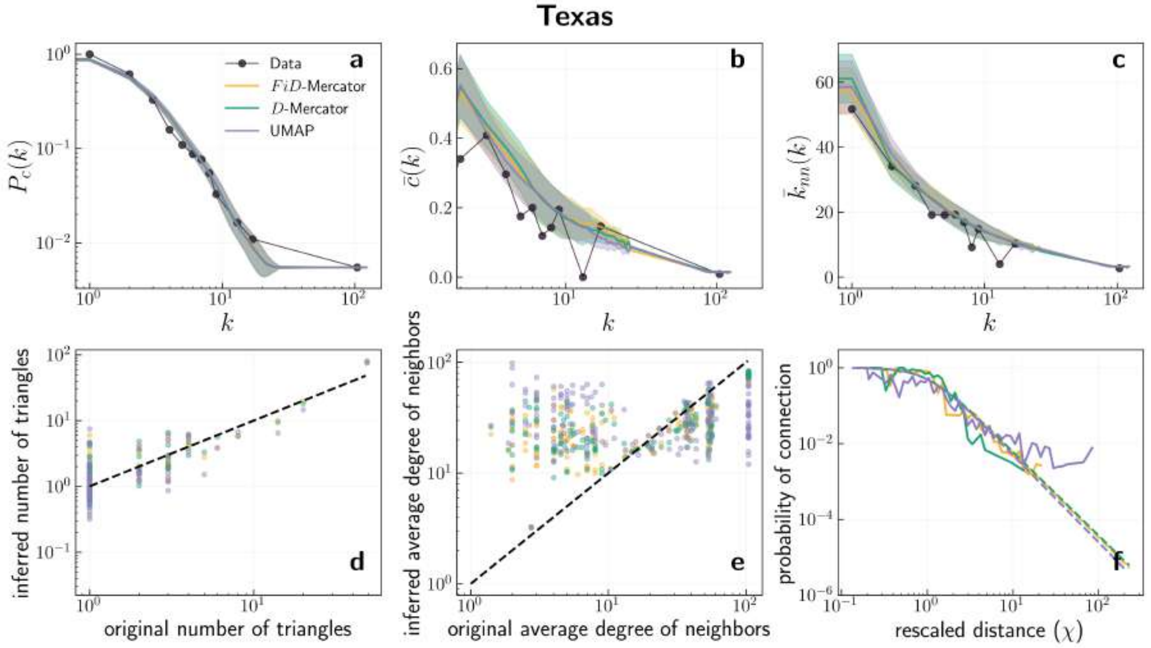


Supplementary Fig. 27: Topological validation of the embeddings of the Texas network. See caption in Supplementary Fig. 21 for more details.

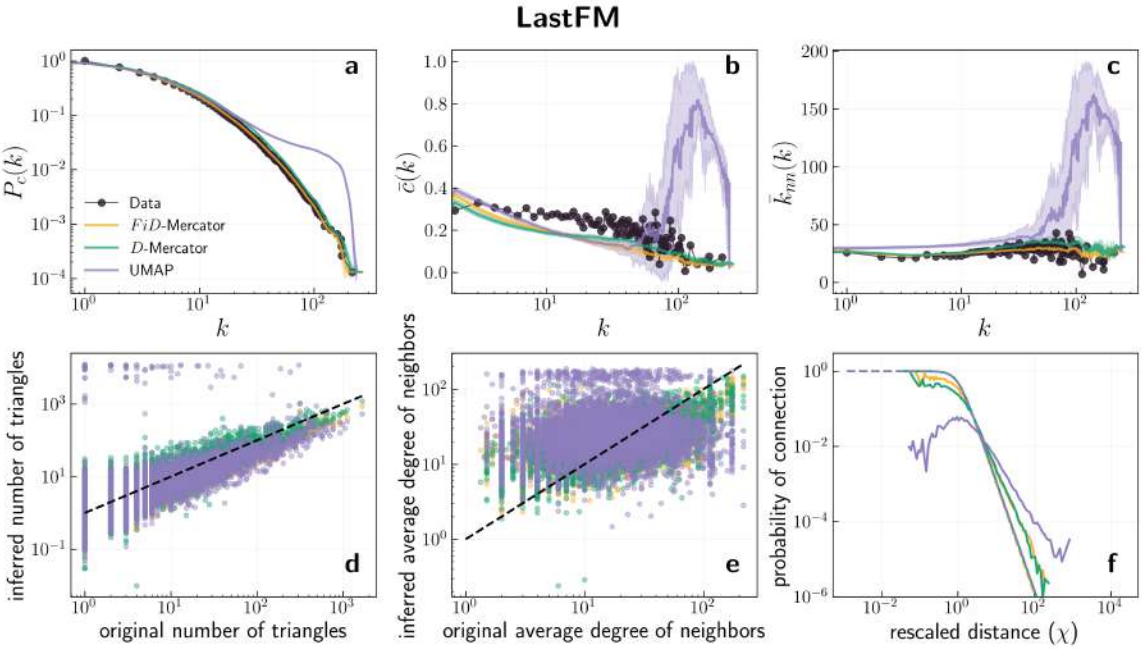


Supplementary Fig. 28: Topological validation of the embeddings of the LastFM network. See caption in Supplementary Fig. 21 for more details.

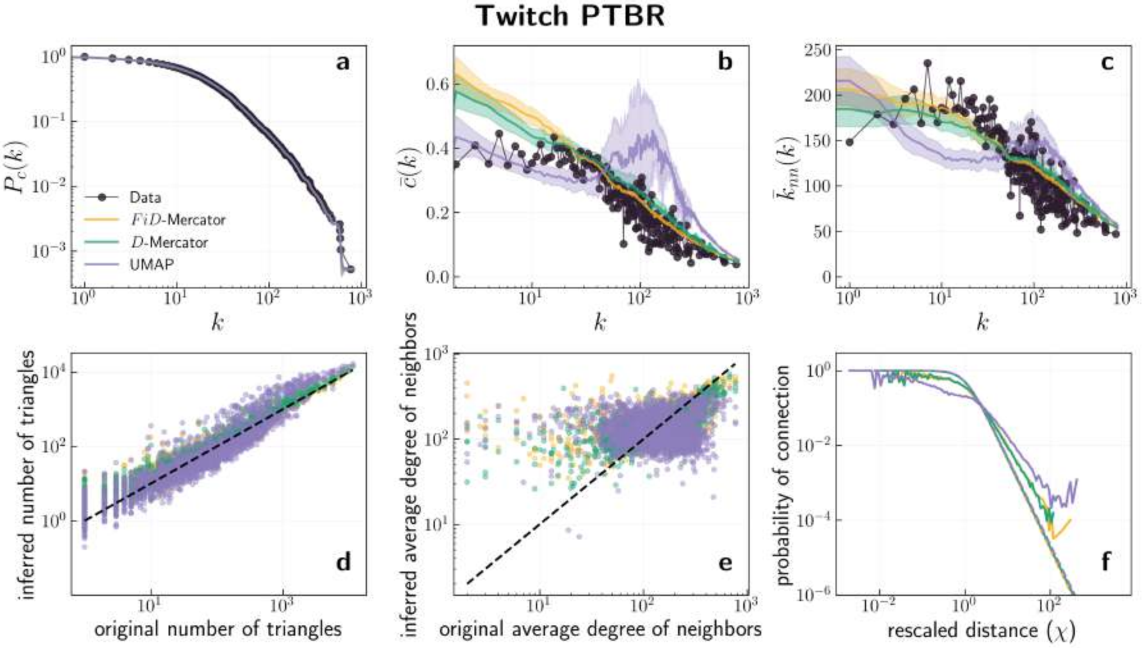


Supplementary Fig. 29: Topological validation of the embeddings of the Twitch PTBR network. See caption in Supplementary Fig. 21 for more details.
